# Supplementary material for: All-electron $\mathrm{\textit{ab-initio}}$ hyperfine coupling of Si-, Ge- and Sn-vacancy defects in diamond
Source: arXiv:2309.13913 source file (2023-09-25)
Supplement: Supplementary file 1 [file Supplementary_Material.pdf]

# Supplemental Material for:

## All-electron ab-initio hyperfine coupling of Si-, Ge- and Sn-vacancy defects in diamond

Akib Karim,[1] Harish H. Vallabhapurapu,[2] Chris Adambukulam,[2]
Arne Laucht,[2] Salvy P. Russo,[3,4] and Alberto Peruzzo[5]

[1] *Quantum Photonics Laboratory and Centre for Quantum Computation and Communication Technology, School of Engineering, RMIT University, Melbourne, VIC 3000, Australia*

[2] *School of Electrical Engineering and Telecommunications, University of New South Wales, Sydney, New South Wales 2052, Australia*

[3] *ARC Centre of Excellence in Exciton Science, School of Science, RMIT University, Melbourne, VIC 3001 Australia*

[4] *Chemical and Quantum Physics, School of Science, RMIT University, Melbourne VIC 3001, Australia*

[5] *Quantum Photonics Laboratory and Centre for Quantum Computation and Communication Technology, School of Engineering, RMIT University, Melbourne, Victoria 3000, Australia*

We report the isotropic and anisotropic values for the hyperfine tensor with each lattice site for 13C for the diamond defects studied in this work. Furthermore, we report the elements of the rotation matrix to rotate from from Cartesian to principal axes for the hyperfine tensor with each lattice site for $^{13}$C for the diamond defects under study.

| Symmetry reduced # | Total # | Atom | x [Å] | y [Å] | z [Å] | Fermi [MHz] | $A_{xx}$ [MHz] | $A_{yy}$ [MHz] | $A_{zz}$ [MHz] |
|---|---|---|---|---|---|---|---|---|---|
| 1 | 1 | SI | 0.0 | 0.0 | 0.0 | 73.777 | -3.120026 | -3.120026 | 6.240053 |
| 2 | 2 | C | 1.3732 | 2.3784 | 5.2584 | -5.5438 | 1.124322 | -1.813765 | 0.6894424 |
| 3 | 8 | C | 2.7508 | 4.7646 | 9.219 | 0.39122 | 0.3142118 | 0.3998015 | -0.7140133 |
| 4 | 14 | C | 4.1269 | 7.1479 | 13.1266 | 0.069415 | 0.02144867 | 0.1678779 | -0.1893266 |
| 5 | 20 | C | -5.5039 | -9.533 | -14.1062 | 0.062998 | -0.07764404 | 0.1664017 | -0.08875762 |
| 6 | 26 | C | -4.1281 | -7.1501 | -10.2053 | 0.47017 | 0.2023053 | -0.4717714 | 0.2694661 |
| 7 | 32 | C | -2.7558 | -4.7731 | -6.2948 | 6.3813 | 2.098059 | -3.90757 | 1.80951 |
| 8 | 38 | C | -1.476 | -2.5566 | -2.3459 | 66.038 | 23.59237 | -47.14481 | 23.55244 |
| 9 | 44 | C | -1.3731 | -2.3783 | 9.1993 | -0.29207 | 0.1241846 | 0.241059 | -0.3652436 |
| 10 | 50 | C | 4.1228 | 2.3812 | 13.1173 | -0.016129 | 0.03545169 | 0.1079541 | -0.1434058 |
| 11 | 62 | C | -16.517 | 4.7654 | 1.4533 | -0.013207 | -0.07078738 | 0.09707566 | -0.02628828 |
| 12 | 74 | C | -4.1329 | -11.9182 | -10.2161 | 0.063923 | -0.008644993 | -0.1252182 | 0.1338632 |
| 13 | 86 | C | -2.7566 | -9.5435 | -6.324 | 0.7322 | 0.3394675 | -0.7485301 | 0.4090626 |
| 14 | 98 | C | -1.3833 | -7.2116 | -2.4343 | 7.2933 | 2.374694 | -4.965231 | 2.590537 |
| 15 | 110 | C | 0.0112 | -4.8589 | 1.4465 | -3.1779 | 2.544715 | -3.572179 | 1.027463 |
| 16 | 122 | C | 8.2592 | 14.3054 | 1.4515 | -0.015307 | 0.0645089 | -0.07885941 | 0.01435051 |
| 17 | 128 | C | -15.1418 | 2.3823 | 5.3486 | -0.0058927 | -0.09067914 | 0.01317192 | 0.07750723 |
| 18 | 140 | C | -2.757 | -14.3046 | -6.3242 | 0.084329 | 0.01319336 | -0.1487646 | 0.1355712 |
| 19 | 152 | C | -1.3787 | -11.9397 | -2.4328 | 0.84342 | 0.4010973 | -0.7647533 | 0.363656 |
| 20 | 164 | C | 0.0007 | -9.5726 | 1.4589 | 0.80257 | 0.6643643 | -1.168272 | 0.503908 |
| 21 | 176 | C | 1.3793 | -7.1671 | 5.344 | -0.94593 | 0.3623908 | -0.6456834 | 0.2832925 |
| 22 | 188 | C | 6.8823 | 11.9205 | 9.2429 | 0.0011938 | -0.021266 | -0.07168705 | 0.09295306 |
| 23 | 194 | C | -1.3788 | -16.6887 | -2.4312 | 0.10026 | 0.1551096 | -0.1658022 | 0.0106926 |
| 24 | 206 | C | 0.0004 | -14.3137 | 1.4601 | 0.17238 | 0.2009871 | -0.2736036 | 0.07261644 |
| 25 | 218 | C | 1.3792 | -11.926 | 5.3512 | -0.11481 | 0.06130411 | -0.2227573 | 0.1614532 |
| 26 | 230 | C | 2.7556 | -9.5364 | 9.2399 | -0.093147 | 0.03963256 | -0.2021809 | 0.1625483 |
| 27 | 242 | C | -6.8836 | -11.9228 | -6.3232 | 0.26859 | 0.1331983 | -0.3052284 | 0.1720302 |
| 28 | 248 | C | 15.145 | 2.3832 | -2.428 | 0.09545 | -0.187261 | 0.1216212 | 0.06563975 |
| 29 | 260 | C | -5.4982 | 4.7651 | -14.0981 | -0.0040303 | -0.09605741 | 0.1188051 | -0.0227477 |
| 30 | 272 | C | 2.7483 | 4.7602 | -14.0956 | -0.0048205 | 0.09865579 | -0.1231457 | 0.02448995 |
| 31 | 278 | C | -4.1238 | 2.3812 | -10.1912 | 0.01669 | 0.1917987 | 0.1159114 | -0.3077101 |
| 32 | 290 | C | 1.3743 | 2.3804 | -6.258 | 1.8569 | -0.5483651 | 1.197566 | -0.6492008 |
| 33 | 296 | C | 0.0 | 0.0 | 13.1111 | -0.031033 | 0.07110092 | 0.07110092 | -0.1422018 |
| 34 | 298 | C | 1.3746 | 2.3809 | 17.0157 | -0.0039648 | -0.01078011 | 0.04183247 | -0.03105237 |
| 35 | 304 | C | -8.2576 | -14.3026 | -10.2188 | 0.03341 | -0.01804618 | -0.05045571 | 0.06850189 |
| 36 | 310 | C | -5.514 | -9.5506 | -2.431 | 0.83936 | 0.428938 | -0.8651279 | 0.4361899 |
| 37 | 316 | C | -4.1383 | -7.1678 | 1.4571 | -0.16243 | 0.3025523 | -0.4079354 | 0.1053831 |
| 38 | 322 | C | -2.7555 | -4.7727 | 5.3305 | -0.34885 | 0.307335 | 0.4401556 | -0.7474905 |
| 39 | 328 | C | 9.6329 | 16.6846 | 5.3472 | 0.0040261 | -0.005198936 | -0.02856439 | 0.03376333 |
| 40 | 334 | C | -6.8832 | -16.6848 | -6.3229 | 0.037062 | 0.009850259 | -0.07291394 | 0.06306368 |
| 41 | 346 | C | -4.1326 | -11.9278 | 1.4625 | 0.02401 | 0.1588118 | -0.2169793 | 0.0581675 |
| 42 | 358 | C | -2.7529 | -9.5397 | 5.3492 | -0.017708 | 0.1388823 | -0.3540801 | 0.2151978 |
| 43 | 370 | C | -1.3746 | -7.1489 | 9.232 | -0.027532 | 0.13552 | 0.1935844 | -0.3291044 |
| 44 | 382 | C | -2.7498 | -4.7628 | -17.9932 | 0.013461 | -0.06532515 | 0.07825894 | -0.01293379 |
| 45 | 388 | C | 8.2562 | 4.7624 | -10.2111 | 0.029846 | 0.1712569 | -0.2131428 | 0.04188583 |
| 46 | 400 | C | 9.6366 | 7.1502 | -6.3247 | 0.021653 | 0.06704039 | -0.2506836 | 0.1836432 |
| 47 | 412 | C | 11.0137 | 9.538 | -2.4368 | -0.030116 | 0.1419069 | -0.1555506 | 0.01364378 |
| 48 | 424 | C | 4.1258 | 7.1462 | -10.209 | 0.024374 | 0.1068543 | -0.2765071 | 0.1696528 |
| 49 | 430 | C | -6.8845 | 2.3861 | -6.3145 | 0.31711 | -0.4376973 | 0.001766656 | 0.4359306 |
| 50 | 442 | C | 2.7635 | 4.7865 | -2.4232 | 0.67114 | -0.5199559 | -0.4076411 | 0.927597 |
| 51 | 448 | C | -0.0 | 0.0 | -21.8894 | 0.016939 | -0.01978652 | -0.01978652 | 0.03957304 |
| 52 | 450 | C | 1.3742 | 2.3802 | -17.9918 | 0.015546 | 0.03660584 | -0.04214495 | 0.00553911 |
| 53 | 456 | C | 5.5053 | 9.5355 | -6.3246 | 0.024821 | 0.1126623 | -0.3233947 | 0.2107324 |
| 54 | 462 | C | 6.8841 | 11.9236 | -2.4386 | -0.020684 | 0.1363532 | -0.199017 | 0.0626638 |
| 55 | 468 | C | -1.3744 | -2.3805 | -14.0913 | -0.0035842 | 0.02910969 | 0.0808719 | -0.1099816 |
| 56 | 474 | C | 6.8925 | 7.1611 | -2.4321 | -0.080544 | 0.1513507 | -0.3570019 | 0.2056512 |
| 57 | 486 | C | 8.2653 | 9.544 | 1.457 | -0.1393 | 0.149464 | -0.2353978 | 0.08593375 |
| 58 | 498 | C | 4.1424 | 7.1749 | 1.4595 | -1.1249 | 0.395299 | -0.7075383 | 0.3122392 |
| 59 | 504 | C | 0.0 | 0.0 | -10.1807 | 0.017999 | 0.1815834 | 0.1815834 | -0.3631668 |
| 60 | 506 | C | 5.509 | 9.5419 | 5.3499 | -0.078839 | 0.1393704 | -0.3134315 | 0.1740611 |

TABLE S1. Isotropic and anisotropic values for the hyperfine tensor with each lattice site for $^{13}C$ for the $SiV^0$ defect in diamond.

| Symmetry reduced # | Total # | Atom | x [Å] | y [Å] | z [Å] | Fermi [MHz] | $A_{xx}$ [MHz] | $A_{yy}$ [MHz] | $A_{zz}$ [MHz] |
|---|---|---|---|---|---|---|---|---|---|
| 1 | 1 | SI | 0.0 | 0.0 | 0.0 | 69.223 | -1.493529 | -1.493529 | 2.987057 |
| 2 | 2 | C | 1.3735 | 2.3789 | 5.243 | -5.5998 | 0.5584253 | -0.9019446 | 0.3435193 |
| 3 | 8 | C | 2.751 | 4.7648 | 9.2154 | 0.36701 | 0.1500447 | 0.1946745 | -0.3447192 |
| 4 | 14 | C | 4.1268 | 7.1479 | 13.1258 | 0.06603 | 0.008678447 | 0.08243471 | -0.09111315 |
| 5 | 20 | C | -5.5039 | -9.533 | -14.1061 | 0.057319 | -0.03675162 | 0.0805972 | -0.04384557 |
| 6 | 26 | C | -4.1277 | -7.1493 | -10.2045 | 0.44491 | 0.09565038 | -0.225968 | 0.1303176 |
| 7 | 32 | C | -2.7532 | -4.7687 | -6.2914 | 6.2566 | 1.018637 | -1.893791 | 0.8751538 |
| 8 | 38 | C | -1.4653 | -2.538 | -2.3252 | 71.145 | 11.8351 | -23.60668 | 11.77158 |
| 9 | 44 | C | -1.3727 | -2.3775 | 9.1929 | -0.27912 | 0.06900861 | 0.1225952 | -0.1916038 |
| 10 | 50 | C | 4.1225 | 2.381 | 13.1151 | -0.012318 | 0.01809513 | 0.05470442 | -0.07279956 |
| 11 | 62 | C | -16.5172 | 4.7653 | 1.4526 | -0.0080092 | -0.03437233 | 0.04799359 | -0.01362126 |
| 12 | 74 | C | -4.1329 | -11.918 | -10.2161 | 0.060783 | -0.004513239 | -0.06064365 | 0.06515689 |
| 13 | 86 | C | -2.756 | -9.5424 | -6.3233 | 0.72198 | 0.1621316 | -0.3591841 | 0.1970526 |
| 14 | 98 | C | -1.3801 | -7.212 | -2.4313 | 7.2156 | 1.154845 | -2.412327 | 1.257483 |
| 15 | 110 | C | 0.0203 | -4.8584 | 1.4497 | -3.0542 | 1.27708 | -1.774385 | 0.497305 |
| 16 | 122 | C | 8.2594 | 14.3056 | 1.4505 | -0.0077728 | 0.03228074 | -0.03861808 | 0.006337334 |
| 17 | 128 | C | -15.1418 | 2.3822 | 5.3483 | 0.0011624 | -0.04307718 | 0.006259511 | 0.03681767 |
| 18 | 140 | C | -2.7569 | -14.3046 | -6.3241 | 0.078394 | 0.005912192 | -0.07101762 | 0.06510543 |
| 19 | 152 | C | -1.3781 | -11.9411 | -2.4323 | 0.81401 | 0.1908939 | -0.3616679 | 0.170774 |
| 20 | 164 | C | 0.0021 | -9.5747 | 1.4595 | 0.71879 | 0.3157917 | -0.5523392 | 0.2365476 |
| 21 | 176 | C | 1.3798 | -7.1666 | 5.3421 | -0.90437 | 0.1795225 | -0.3247742 | 0.1452518 |
| 22 | 188 | C | 6.8823 | 11.9205 | 9.2427 | -5.7282e-05 | -0.009723188 | -0.03504059 | 0.04476378 |
| 23 | 194 | C | -1.3788 | -16.6893 | -2.431 | 0.09583 | 0.07513384 | -0.07754621 | 0.002412375 |
| 24 | 206 | C | 0.0007 | -14.3149 | 1.4603 | 0.16115 | 0.09721127 | -0.1292549 | 0.03204359 |
| 25 | 218 | C | 1.3792 | -11.9262 | 5.3511 | -0.10748 | 0.03113996 | -0.110631 | 0.07949102 |
| 26 | 230 | C | 2.7556 | -9.5363 | 9.2393 | -0.091335 | 0.01979633 | -0.1006222 | 0.08082583 |
| 27 | 242 | C | -6.8834 | -11.9225 | -6.3228 | 0.25338 | 0.06170304 | -0.1417534 | 0.08005035 |
| 28 | 248 | C | 15.145 | 2.3832 | -2.4273 | 0.088427 | -0.08774971 | 0.05830098 | 0.02944873 |
| 29 | 260 | C | -5.4979 | 4.7648 | -14.0971 | -0.0046397 | -0.04880518 | 0.0593695 | -0.01056432 |
| 30 | 272 | C | 2.7482 | 4.76 | -14.0943 | -0.0070336 | 0.0495981 | -0.0624285 | 0.01283041 |
| 31 | 278 | C | -4.1228 | 2.3807 | -10.1884 | 0.0093407 | 0.09605711 | 0.06050561 | -0.1565627 |
| 32 | 290 | C | 1.372 | 2.3764 | -6.2499 | 1.8054 | -0.2428048 | 0.5986281 | -0.3558233 |
| 33 | 296 | C | 0.0 | 0.0 | 13.1078 | -0.024629 | 0.03639296 | 0.03639296 | -0.07278592 |
| 34 | 298 | C | 1.3745 | 2.3808 | 17.0144 | -0.0021497 | -0.004588009 | 0.02117169 | -0.01658368 |
| 35 | 304 | C | -8.2576 | -14.3026 | -10.2191 | 0.033634 | -0.008666399 | -0.0234157 | 0.03208209 |
| 36 | 310 | C | -5.5136 | -9.5498 | -2.43 | 0.81267 | 0.2038553 | -0.4095026 | 0.2056473 |
| 37 | 316 | C | -4.1365 | -7.1646 | 1.457 | -0.1725 | 0.1576471 | -0.2167573 | 0.05911024 |
| 38 | 322 | C | -2.7541 | -4.7703 | 5.3267 | -0.29854 | 0.1686947 | 0.2253778 | -0.3940725 |
| 39 | 328 | C | 9.6329 | 16.6847 | 5.3468 | 0.0068964 | -0.001309778 | -0.01262508 | 0.01393486 |
| 40 | 334 | C | -6.8832 | -16.6847 | -6.3227 | 0.031475 | 0.004477256 | -0.03288455 | 0.02840729 |
| 41 | 346 | C | -4.1324 | -11.9274 | 1.463 | 0.028752 | 0.07955349 | -0.1097661 | 0.03021264 |
| 42 | 358 | C | -2.7526 | -9.5388 | 5.3487 | -0.013531 | 0.07320216 | -0.1814932 | 0.108291 |
| 43 | 370 | C | -1.3745 | -7.1483 | 9.2302 | -0.021972 | 0.06985606 | 0.0978537 | -0.1677098 |
| 44 | 382 | C | -2.7497 | -4.7626 | -17.9925 | 0.0056591 | -0.03010061 | 0.03812458 | -0.008023968 |
| 45 | 388 | C | 8.2557 | 4.7623 | -10.2105 | 0.02318 | 0.08543736 | -0.1084451 | 0.02300774 |
| 46 | 400 | C | 9.6362 | 7.1502 | -6.3247 | 0.019285 | 0.0361914 | -0.1275993 | 0.0914079 |
| 47 | 412 | C | 11.0137 | 9.5382 | -2.4373 | -0.028372 | 0.07130362 | -0.07867571 | 0.007372091 |
| 48 | 424 | C | 4.1257 | 7.1459 | -10.2081 | 0.014456 | 0.05705741 | -0.1413595 | 0.08430212 |
| 49 | 430 | C | -6.8828 | 2.3855 | -6.3128 | 0.30569 | -0.2272795 | 0.01199464 | 0.2152849 |
| 50 | 442 | C | 2.7606 | 4.7816 | -2.421 | 0.64646 | -0.2257823 | -0.2466694 | 0.4724517 |
| 51 | 448 | C | -0.0 | 0.0 | -21.8892 | 0.003831 | -0.008236307 | -0.008236307 | 0.01647261 |
| 52 | 450 | C | 1.3741 | 2.3801 | -17.9909 | 0.0092523 | 0.01827489 | -0.01932816 | 0.001053266 |
| 53 | 456 | C | 5.5052 | 9.5352 | -6.3246 | 0.016718 | 0.06044074 | -0.1655089 | 0.1050682 |
| 54 | 462 | C | 6.8841 | 11.9237 | -2.4393 | -0.006702 | 0.06877844 | -0.101281 | 0.03250257 |
| 55 | 468 | C | -1.3742 | -2.3802 | -14.0894 | -0.0095328 | 0.01490036 | 0.04093956 | -0.05583993 |
| 56 | 474 | C | 6.8919 | 7.1605 | -2.4316 | -0.072808 | 0.07897995 | -0.1840167 | 0.1050367 |
| 57 | 486 | C | 8.2655 | 9.5443 | 1.4568 | -0.13406 | 0.07392599 | -0.1152459 | 0.04131988 |
| 58 | 498 | C | 4.1425 | 7.175 | 1.4593 | -1.1165 | 0.1976204 | -0.3524617 | 0.1548413 |
| 59 | 504 | C | -0.0 | 0.0 | -10.1765 | 0.00037094 | 0.09273835 | 0.09273835 | -0.1854767 |
| 60 | 506 | C | 5.5089 | 9.5417 | 5.3494 | -0.062722 | 0.06699324 | -0.1511849 | 0.08419166 |

TABLE S2. Isotropic and anisotropic values for the hyperfine tensor with each lattice site for $^{13}C$ for the $SiV^{-}$ defect in diamond.

| Symmetry reduced # | Total # | Atom | x [Å] | y [Å] | z [Å] | Fermi [MHz] | $A_{xx}$ [MHz] | $A_{yy}$ [MHz] | $A_{zz}$ [MHz] |
|---|---|---|---|---|---|---|---|---|---|
| 1 | 1 | GE | 0.0 | 0.0 | 0.0 | 44.013 | -1.704648 | -1.704648 | 3.409296 |
| 2 | 2 | C | 1.3777 | 2.3862 | 5.271 | -6.055 | 1.124191 | 0.6709144 | -1.795105 |
| 3 | 8 | C | 2.7526 | 4.7676 | 9.2235 | 0.63573 | 0.3514831 | 0.4304806 | -0.7819638 |
| 4 | 14 | C | 4.1273 | 7.1488 | 13.1278 | 0.093291 | 0.02575542 | 0.1698531 | -0.1956085 |
| 5 | 20 | C | -5.5041 | -9.5334 | -14.1065 | 0.072902 | -0.06389816 | 0.1601247 | -0.0962265 |
| 6 | 26 | C | -4.1291 | -7.1518 | -10.2077 | 0.55334 | 0.2039763 | -0.4792423 | 0.2752659 |
| 7 | 32 | C | -2.7588 | -4.7783 | -6.3028 | 7.7367 | 2.179524 | -4.078656 | 1.899132 |
| 8 | 38 | C | -1.5017 | -2.601 | -2.3766 | 71.791 | 25.47162 | -50.90344 | 25.43182 |
| 9 | 44 | C | -1.3735 | -2.379 | 9.2018 | -0.32692 | 0.1321651 | 0.2448537 | -0.3770188 |
| 10 | 50 | C | 4.1229 | 2.3814 | 13.1184 | -0.013946 | 0.03910776 | 0.1101972 | -0.1493049 |
| 11 | 62 | C | -16.5175 | 4.7654 | 1.4535 | -0.012883 | -0.06527087 | 0.0943056 | -0.02903472 |
| 12 | 74 | C | -4.1337 | -11.9189 | -10.2165 | 0.049912 | -0.009130727 | -0.1144223 | 0.123553 |
| 13 | 86 | C | -2.7573 | -9.5457 | -6.3251 | 0.62903 | 0.2925282 | -0.6481962 | 0.355668 |
| 14 | 98 | C | -1.3835 | -7.2216 | -2.4347 | 7.645 | 2.222988 | -4.662243 | 2.439255 |
| 15 | 110 | C | 0.014 | -4.8722 | 1.4509 | -4.4866 | 2.287713 | -2.969944 | 0.682231 |
| 16 | 122 | C | 8.2596 | 14.3061 | 1.4518 | -0.011819 | 0.06344348 | -0.0752094 | 0.01176592 |
| 17 | 128 | C | -15.1427 | 2.3821 | 5.3487 | -0.0059874 | -0.07992093 | 0.01231146 | 0.06760947 |
| 18 | 140 | C | -2.7578 | -14.3055 | -6.3243 | 0.06618 | 0.01018938 | -0.1299805 | 0.1197912 |
| 19 | 152 | C | -1.3791 | -11.9435 | -2.433 | 0.82404 | 0.3652854 | -0.6879795 | 0.322694 |
| 20 | 164 | C | 0.0011 | -9.5793 | 1.4594 | 0.90442 | 0.6310723 | -1.098129 | 0.4670565 |
| 21 | 176 | C | 1.3801 | -7.171 | 5.3461 | -0.90121 | 0.284649 | -0.6429957 | 0.3583468 |
| 22 | 188 | C | 6.8827 | 11.9212 | 9.2429 | 0.0024747 | -0.01614547 | -0.06858176 | 0.08472723 |
| 23 | 194 | C | -1.3793 | -16.6897 | -2.4311 | 0.094326 | 0.1454314 | -0.1454606 | 2.920595e-05 |
| 24 | 206 | C | 0.0007 | -14.3159 | 1.4601 | 0.17269 | 0.1890406 | -0.2478843 | 0.05884373 |
| 25 | 218 | C | 1.3798 | -11.9279 | 5.3516 | -0.10267 | 0.06553078 | -0.2191451 | 0.1536143 |
| 26 | 230 | C | 2.7563 | -9.5377 | 9.2409 | -0.090868 | 0.04056545 | -0.1995157 | 0.1589503 |
| 27 | 242 | C | -6.8841 | -11.9237 | -6.3234 | 0.22234 | 0.1087052 | -0.2507029 | 0.1419977 |
| 28 | 248 | C | 15.1461 | 2.3832 | -2.4281 | 0.070013 | -0.1534377 | 0.1068796 | 0.04655808 |
| 29 | 260 | C | -5.498 | 4.7653 | -14.0987 | -0.0052853 | -0.1019907 | 0.1188454 | -0.01685476 |
| 30 | 272 | C | 2.7481 | 4.7599 | -14.0963 | -0.0083542 | 0.09857654 | -0.1282081 | 0.02963159 |
| 31 | 278 | C | -4.1244 | 2.3819 | -10.1929 | 0.014797 | 0.1948379 | 0.1261944 | -0.3210323 |
| 32 | 290 | C | 1.3754 | 2.3823 | -6.2614 | 2.2147 | -0.5025431 | 1.207823 | -0.7052803 |
| 33 | 296 | C | 0.0 | 0.0 | 13.1119 | -0.030293 | 0.07397479 | 0.07397479 | -0.1479496 |
| 34 | 298 | C | 1.3745 | 2.3807 | 17.016 | -0.0012552 | -0.006415909 | 0.04312292 | -0.03670701 |
| 35 | 304 | C | -8.2578 | -14.303 | -10.2188 | 0.026786 | -0.01628925 | -0.0418495 | 0.05813875 |
| 36 | 310 | C | -5.5153 | -9.5528 | -2.431 | 0.71367 | 0.3653186 | -0.7296149 | 0.3642964 |
| 37 | 316 | C | -4.1391 | -7.1692 | 1.4576 | -0.20883 | 0.2925645 | -0.402347 | 0.1097825 |
| 38 | 322 | C | -2.7562 | -4.7739 | 5.3319 | -0.39204 | 0.3299765 | 0.4653471 | -0.7953236 |
| 39 | 328 | C | 9.633 | 16.6849 | 5.3473 | 0.00024835 | 0.0008382046 | -0.02111044 | 0.02027224 |
| 40 | 334 | C | -6.8836 | -16.6851 | -6.3229 | 0.024588 | 0.006469555 | -0.0546352 | 0.04816565 |
| 41 | 346 | C | -4.133 | -11.929 | 1.4624 | 0.014418 | 0.1565727 | -0.2204747 | 0.06390198 |
| 42 | 358 | C | -2.753 | -9.5406 | 5.3495 | -0.015011 | 0.1543712 | -0.3718505 | 0.2174793 |
| 43 | 370 | C | -1.3744 | -7.1494 | 9.2328 | -0.025426 | 0.1428786 | 0.2002192 | -0.3430978 |
| 44 | 382 | C | -2.7496 | -4.7625 | -17.9934 | 0.0048894 | -0.05153486 | 0.07324522 | -0.02171036 |
| 45 | 388 | C | 8.2567 | 4.762 | -10.2114 | 0.027282 | 0.1709465 | -0.2233078 | 0.05236132 |
| 46 | 400 | C | 9.6374 | 7.1501 | -6.3248 | 0.016743 | 0.08389827 | -0.262962 | 0.1790638 |
| 47 | 412 | C | 11.0145 | 9.5383 | -2.4367 | -0.025855 | 0.1436539 | -0.1622441 | 0.01859025 |
| 48 | 424 | C | 4.1258 | 7.1461 | -10.2093 | 0.022445 | 0.1177421 | -0.2884474 | 0.1707053 |
| 49 | 430 | C | -6.8857 | 2.3868 | -6.3154 | 0.32122 | -0.4628357 | 0.03470673 | 0.428129 |
| 50 | 442 | C | 2.7641 | 4.7876 | -2.4254 | 0.8878 | -0.4091758 | -0.5085823 | 0.9177581 |
| 51 | 448 | C | 0.0 | 0.0 | -21.8894 | 0.0098625 | -0.01168558 | -0.01168558 | 0.02337115 |
| 52 | 450 | C | 1.374 | 2.3799 | -17.992 | 0.010061 | 0.03581134 | -0.03329129 | -0.002520055 |
| 53 | 456 | C | 5.5055 | 9.5357 | -6.3247 | 0.019837 | 0.1281506 | -0.3376627 | 0.2095121 |
| 54 | 462 | C | 6.8845 | 11.9243 | -2.4383 | -0.012797 | 0.1370923 | -0.2071209 | 0.0700286 |
| 55 | 468 | C | -1.3744 | -2.3805 | -14.092 | 0.0020897 | 0.03272663 | 0.08207066 | -0.1147973 |
| 56 | 474 | C | 6.894 | 7.1623 | -2.4324 | -0.058049 | 0.1689031 | -0.3778924 | 0.2089893 |
| 57 | 486 | C | 8.2666 | 9.5455 | 1.4572 | -0.12563 | 0.1433733 | -0.2197397 | 0.07636635 |
| 58 | 498 | C | 4.1446 | 7.1787 | 1.4595 | -1.0535 | 0.395128 | -0.6651469 | 0.270019 |
| 59 | 504 | C | -0.0 | 0.0 | -10.1821 | 0.039103 | 0.1844403 | 0.1844403 | -0.3688806 |
| 60 | 506 | C | 5.5099 | 9.5434 | 5.3503 | -0.039814 | 0.1293028 | -0.2895257 | 0.1602229 |

TABLE S3. Isotropic and anisotropic values for the hyperfine tensor with each lattice site for $^{13}C$ for the $GeV^0$ defect in diamond.

| Symmetry reduced # | Total # | Atom | x [Å] | y [Å] | z [Å] | Fermi [MHz] | $A_{xx}$ [MHz] | $A_{yy}$ [MHz] | $A_{zz}$ [MHz] |
|---|---|---|---|---|---|---|---|---|---|
| 1 | 1 | GE | 0.0 | 0.0 | 0.0 | 42.458 | 0.8311744 | 0.8311744 | -1.662349 |
| 2 | 2 | C | 1.3789 | 2.3883 | 5.2589 | -6.1642 | -0.5585947 | -0.3266363 | 0.8852309 |
| 3 | 8 | C | 2.7532 | 4.7687 | 9.2216 | 0.60421 | -0.1694645 | -0.2104267 | 0.3798912 |
| 4 | 14 | C | 4.1275 | 7.149 | 13.1276 | 0.092761 | -0.01110757 | -0.08356139 | 0.09466896 |
| 5 | 20 | C | -5.5041 | -9.5334 | -14.1065 | 0.063498 | 0.03064928 | -0.07815793 | 0.04750865 |
| 6 | 26 | C | -4.1289 | -7.1515 | -10.2079 | 0.52535 | -0.09759915 | 0.2320749 | -0.1344757 |
| 7 | 32 | C | -2.7569 | -4.775 | -6.3025 | 7.7651 | -1.068603 | 1.999104 | -0.9305008 |
| 8 | 38 | C | -1.496 | -2.5912 | -2.366 | 75.234 | -12.71399 | 25.38322 | -12.66924 |
| 9 | 44 | C | -1.3732 | -2.3785 | 9.1964 | -0.32937 | -0.07142738 | -0.1247426 | 0.1961699 |
| 10 | 50 | C | 4.1227 | 2.3812 | 13.1167 | -0.012482 | -0.01980602 | -0.05553018 | 0.0753362 |
| 11 | 62 | C | -16.5178 | 4.7653 | 1.453 | -0.010618 | 0.03217334 | -0.0468888 | 0.01471546 |
| 12 | 74 | C | -4.1338 | -11.9187 | -10.2164 | 0.045892 | 0.004593132 | 0.05607653 | -0.06066966 |
| 13 | 86 | C | -2.7568 | -9.5448 | -6.3246 | 0.61163 | -0.1405123 | 0.3125204 | -0.1720081 |
| 14 | 98 | C | -1.3805 | -7.2233 | -2.4319 | 7.6415 | -1.082768 | 2.268699 | -1.185931 |
| 15 | 110 | C | 0.0229 | -4.8715 | 1.4549 | -4.5636 | -1.1405 | 1.45699 | -0.3164896 |
| 16 | 122 | C | 8.2597 | 14.3062 | 1.4511 | -0.013633 | -0.0317168 | 0.03726168 | -0.005544877 |
| 17 | 128 | C | -15.1427 | 2.3821 | 5.3485 | -0.0047303 | 0.03880181 | -0.006050788 | -0.03275102 |
| 18 | 140 | C | -2.7578 | -14.3055 | -6.3243 | 0.062137 | -0.00489144 | 0.06303117 | -0.05813973 |
| 19 | 152 | C | -1.3784 | -11.9452 | -2.4326 | 0.78742 | -0.1748764 | 0.3270594 | -0.1521831 |
| 20 | 164 | C | 0.0024 | -9.582 | 1.46 | 0.79953 | -0.3013767 | 0.5218257 | -0.220449 |
| 21 | 176 | C | 1.3806 | -7.1707 | 5.3449 | -0.91217 | -0.1456461 | 0.324263 | -0.1786169 |
| 22 | 188 | C | 6.8827 | 11.9212 | 9.2428 | 0.00024022 | 0.007523895 | 0.03393423 | -0.04145813 |
| 23 | 194 | C | -1.3792 | -16.6903 | -2.4309 | 0.087383 | -0.07095688 | 0.06870455 | 0.002252329 |
| 24 | 206 | C | 0.0009 | -14.3173 | 1.4604 | 0.16041 | -0.09207479 | 0.1182319 | -0.02615708 |
| 25 | 218 | C | 1.3799 | -11.9282 | 5.3516 | -0.10225 | -0.03323222 | 0.1093233 | -0.07609107 |
| 26 | 230 | C | 2.7565 | -9.5377 | 9.2406 | -0.086763 | -0.02043458 | 0.09964959 | -0.07921501 |
| 27 | 242 | C | -6.884 | -11.9234 | -6.323 | 0.212 | -0.05077639 | 0.1175412 | -0.06676485 |
| 28 | 248 | C | 15.1461 | 2.3832 | -2.4276 | 0.063176 | 0.07277976 | -0.05183296 | -0.0209468 |
| 29 | 260 | C | -5.4977 | 4.7651 | -14.098 | -0.0079296 | 0.05158236 | -0.05948856 | 0.007906199 |
| 30 | 272 | C | 2.7481 | 4.7598 | -14.0954 | -0.0069103 | -0.04950928 | 0.06470177 | -0.01519249 |
| 31 | 278 | C | -4.1236 | 2.3815 | -10.191 | 0.014689 | -0.09773909 | -0.0647394 | 0.1624785 |
| 32 | 290 | C | 1.3734 | 2.3788 | -6.2549 | 2.1936 | 0.2321209 | -0.6067724 | 0.3746515 |
| 33 | 296 | C | 0.0 | 0.0 | 13.1092 | -0.035151 | -0.03761896 | -0.03761896 | 0.07523793 |
| 34 | 298 | C | 1.3745 | 2.3806 | 17.015 | -0.0034676 | 0.002728063 | -0.02181898 | 0.01909092 |
| 35 | 304 | C | -8.2579 | -14.303 | -10.219 | 0.022365 | 0.008009545 | 0.01982878 | -0.02783832 |
| 36 | 310 | C | -5.5149 | -9.5521 | -2.4301 | 0.68493 | -0.1747248 | 0.3476278 | -0.1729031 |
| 37 | 316 | C | -4.1373 | -7.1659 | 1.4576 | -0.2188 | -0.1506422 | 0.2118743 | -0.06123203 |
| 38 | 322 | C | -2.7548 | -4.7715 | 5.3286 | -0.3761 | -0.1757443 | -0.2371783 | 0.4129226 |
| 39 | 328 | C | 9.6331 | 16.6849 | 5.347 | 0.0016775 | -0.001247765 | 0.009711843 | -0.008464078 |
| 40 | 334 | C | -6.8836 | -16.685 | -6.3228 | 0.022983 | -0.002622562 | 0.02496365 | -0.02234109 |
| 41 | 346 | C | -4.1328 | -11.9285 | 1.4628 | 0.012993 | -0.07840882 | 0.1113381 | -0.03292925 |
| 42 | 358 | C | -2.7527 | -9.5397 | 5.3491 | -0.019059 | -0.07967451 | 0.1889687 | -0.1092942 |
| 43 | 370 | C | -1.3744 | -7.1489 | 9.2313 | -0.022527 | -0.07274859 | -0.1008901 | 0.1736387 |
| 44 | 382 | C | -2.7495 | -4.7624 | -17.9928 | 0.0057183 | 0.02410246 | -0.03603334 | 0.01193089 |
| 45 | 388 | C | 8.2563 | 4.762 | -10.211 | 0.024677 | -0.08539005 | 0.112857 | -0.02746692 |
| 46 | 400 | C | 9.637 | 7.1501 | -6.3247 | 0.016828 | -0.04356179 | 0.1327703 | -0.0892085 |
| 47 | 412 | C | 11.0145 | 9.5385 | -2.437 | -0.025369 | -0.07207826 | 0.08177967 | -0.009701412 |
| 48 | 424 | C | 4.1257 | 7.1459 | -10.2087 | 0.022437 | -0.06153571 | 0.1464513 | -0.08491558 |
| 49 | 430 | C | -6.8841 | 2.3862 | -6.314 | 0.31187 | 0.2380544 | -0.02570445 | -0.21235 |
| 50 | 442 | C | 2.7612 | 4.7826 | -2.4236 | 0.8833 | 0.1792516 | 0.2878409 | -0.4670925 |
| 51 | 448 | C | 0.0 | 0.0 | -21.8893 | 0.0083138 | 0.004863602 | 0.004863602 | -0.009727204 |
| 52 | 450 | C | 1.374 | 2.3798 | -17.9913 | 0.0084168 | -0.01789308 | 0.01593443 | 0.001958655 |
| 53 | 456 | C | 5.5053 | 9.5355 | -6.3246 | 0.018608 | -0.06694574 | 0.1714371 | -0.1044914 |
| 54 | 462 | C | 6.8845 | 11.9243 | -2.4388 | -0.013747 | -0.06889347 | 0.1047528 | -0.03585936 |
| 55 | 468 | C | -1.3743 | -2.3803 | -14.0905 | -0.00061175 | -0.01666622 | -0.04142397 | 0.05809019 |
| 56 | 474 | C | 6.8934 | 7.1616 | -2.432 | -0.060426 | -0.08682618 | 0.1930018 | -0.1061756 |
| 57 | 486 | C | 8.2668 | 9.5458 | 1.4571 | -0.11887 | -0.07139515 | 0.1087098 | -0.03731466 |
| 58 | 498 | C | 4.1448 | 7.1789 | 1.4591 | -1.0719 | -0.1988142 | 0.3336077 | -0.1347935 |
| 59 | 504 | C | -0.0 | 0.0 | -10.1787 | 0.027581 | -0.09375011 | -0.09375011 | 0.1875002 |
| 60 | 506 | C | 5.5098 | 9.5432 | 5.3499 | -0.039707 | -0.06310904 | 0.1414104 | -0.07830138 |

TABLE S4. Isotropic and anisotropic values for the hyperfine tensor with each lattice site for $^{13}C$ for the $GeV^{-}$ defect in diamond.

| Symmetry reduced # | Total # | Atom | x [Å] | y [Å] | z [Å] | Fermi [MHz] | $A_{xx}$ [MHz] | $A_{yy}$ [MHz] | $A_{zz}$ [MHz] |
|---|---|---|---|---|---|---|---|---|---|
| 1 | 1 | SN117 | 0.0 | 0.0 | 0.0 | 576.26 | 28.53777 | 28.53777 | -57.07554 |
| 1 | 1 | SN119 | 0.0 | 0.0 | 0.0 | 602.88 | 29.85612 | 29.85612 | -59.71224 |
| 2 | 2 | C | 1.3908 | 2.4089 | 5.3093 | -6.375 | -1.194907 | -0.5097203 | 1.704627 |
| 3 | 8 | C | 2.7577 | 4.7765 | 9.2392 | 0.9383 | -0.4087843 | -0.4790716 | 0.887856 |
| 4 | 14 | C | 4.1287 | 7.1512 | 13.1323 | 0.11653 | -0.03390818 | -0.1762468 | 0.210155 |
| 5 | 20 | C | -5.5046 | -9.5343 | -14.1078 | 0.083876 | 0.05384573 | -0.1611227 | 0.107277 |
| 6 | 26 | C | -4.132 | -7.1569 | -10.2164 | 0.64528 | -0.2194084 | 0.5113576 | -0.2919493 |
| 7 | 32 | C | -2.7671 | -4.7927 | -6.3317 | 9.3449 | -2.316649 | 4.358127 | -2.041477 |
| 8 | 38 | C | -1.5554 | -2.694 | -2.4667 | 62.205 | -26.35778 | 52.83907 | -26.48128 |
| 9 | 44 | C | -1.3749 | -2.3814 | 9.2111 | -0.33136 | -0.129735 | -0.2519838 | 0.3817188 |
| 10 | 50 | C | 4.1234 | 2.3818 | 13.1228 | -0.0096218 | -0.04221199 | -0.1115566 | 0.1537686 |
| 11 | 62 | C | -16.5187 | 4.7653 | 1.4547 | -0.0068461 | 0.06267539 | -0.09299729 | 0.0303219 |
| 12 | 74 | C | -4.1356 | -11.9205 | -10.2174 | 0.036339 | 0.008952359 | 0.1081944 | -0.1171468 |
| 13 | 86 | C | -2.759 | -9.5511 | -6.3289 | 0.4807 | -0.2551523 | 0.5645446 | -0.3093923 |
| 14 | 98 | C | -1.3844 | -7.2453 | -2.4378 | 7.6397 | -2.05003 | 4.340139 | -2.290109 |
| 15 | 110 | C | 0.0194 | -4.9003 | 1.4642 | -5.4007 | -2.120443 | 2.529531 | -0.4090879 |
| 16 | 122 | C | 8.2603 | 14.3072 | 1.4537 | -0.01771 | -0.06247151 | 0.07344742 | -0.01097591 |
| 17 | 128 | C | -15.1445 | 2.3817 | 5.3492 | -0.0047782 | 0.07523948 | -0.01225721 | -0.06298227 |
| 18 | 140 | C | -2.7598 | -14.3075 | -6.3246 | 0.050714 | -0.009810519 | 0.1200876 | -0.1102771 |
| 19 | 152 | C | -1.38 | -11.9523 | -2.4342 | 0.80566 | -0.346085 | 0.6476306 | -0.3015456 |
| 20 | 164 | C | 0.0013 | -9.5945 | 1.4604 | 1.0701 | -0.6328605 | 1.101114 | -0.4682534 |
| 21 | 176 | C | 1.3818 | -7.1792 | 5.3538 | -0.75229 | -0.2841064 | 0.6503883 | -0.3662819 |
| 22 | 188 | C | 6.8836 | 11.9227 | 9.2433 | -0.0072942 | 0.01326259 | 0.06761652 | -0.08087911 |
| 23 | 194 | C | -1.3804 | -16.6918 | -2.4309 | 0.089308 | -0.1413533 | 0.1368492 | 0.004504073 |
| 24 | 206 | C | 0.0012 | -14.3209 | 1.4601 | 0.16896 | -0.1840714 | 0.2359331 | -0.05186169 |
| 25 | 218 | C | 1.3812 | -11.9319 | 5.3529 | -0.085393 | -0.1491942 | 0.2170219 | -0.06782773 |
| 26 | 230 | C | 2.7582 | -9.5405 | 9.2443 | -0.087351 | -0.0427712 | 0.1996835 | -0.1569123 |
| 27 | 242 | C | -6.8854 | -11.9258 | -6.3242 | 0.19893 | -0.09417991 | 0.2192682 | -0.1250883 |
| 28 | 248 | C | 15.1485 | 2.3833 | -2.4293 | 0.055669 | 0.1329861 | -0.09778975 | -0.03519638 |
| 29 | 260 | C | -5.4976 | 4.7662 | -14.1013 | -0.012624 | 0.1058745 | -0.1193844 | 0.01350986 |
| 30 | 272 | C | 2.7478 | 4.7594 | -14.0995 | -0.016221 | -0.0979643 | -0.03250928 | 0.1304736 |
| 31 | 278 | C | -4.1265 | 2.3838 | -10.2003 | 0.0067868 | -0.1989239 | -0.1289833 | 0.3279072 |
| 32 | 290 | C | 1.3783 | 2.3873 | -6.2759 | 2.5808 | 0.6555556 | -1.269273 | 0.6137171 |
| 33 | 296 | C | 0.0 | 0.0 | 13.1158 | -0.024234 | -0.07547276 | -0.07547276 | 0.1509455 |
| 34 | 298 | C | 1.3744 | 2.3804 | 17.0179 | -0.0064145 | 0.004090176 | -0.04356917 | 0.03947899 |
| 35 | 304 | C | -8.2584 | -14.3039 | -10.2185 | 0.01873 | 0.01560542 | 0.03763495 | -0.05324037 |
| 36 | 310 | C | -5.5184 | -9.5581 | -2.432 | 0.54839 | -0.3153009 | 0.6250256 | -0.3097247 |
| 37 | 316 | C | -4.142 | -7.1742 | 1.4585 | -0.18605 | -0.2779164 | 0.3985597 | -0.1206433 |
| 38 | 322 | C | -2.7579 | -4.7769 | 5.3383 | -0.45323 | -0.3162057 | 0.7837031 | -0.4674974 |
| 39 | 328 | C | 9.6333 | 16.6854 | 5.3479 | 0.0044879 | -0.003843612 | 0.01778031 | -0.01393669 |
| 40 | 334 | C | -6.8845 | -16.6857 | -6.3233 | 0.019072 | -0.003831969 | 0.04532664 | -0.04149467 |
| 41 | 346 | C | -4.134 | -11.9319 | 1.4616 | 0.019411 | -0.1549222 | 0.2224994 | -0.06757725 |
| 42 | 358 | C | -2.753 | -9.5427 | 5.3505 | -0.0071402 | -0.1593246 | 0.3761965 | -0.216872 |
| 43 | 370 | C | -1.3741 | -7.1508 | 9.2363 | -0.020494 | -0.1454058 | -0.2037852 | 0.349191 |
| 44 | 382 | C | -2.7493 | -4.7619 | -17.9944 | 0.0023212 | 0.04410902 | -0.070515 | 0.02640598 |
| 45 | 388 | C | 8.2582 | 4.7614 | -10.2133 | 0.023523 | -0.1721495 | 0.2284484 | -0.05629894 |
| 46 | 400 | C | 9.6393 | 7.15 | -6.3249 | 0.024742 | -0.09287485 | 0.2683006 | -0.1754257 |
| 47 | 412 | C | 11.0164 | 9.539 | -2.4354 | -0.028444 | -0.1448787 | 0.1658968 | -0.0210181 |
| 48 | 424 | C | 4.1258 | 7.1461 | -10.2115 | 0.021644 | -0.1189195 | 0.2920121 | -0.1730926 |
| 49 | 430 | C | -6.8887 | 2.3885 | -6.3195 | 0.31269 | 0.4689521 | -0.04243157 | -0.4265206 |
| 50 | 442 | C | 2.7685 | 4.7952 | -2.4323 | 0.82001 | 0.4010443 | 0.4858234 | -0.8868678 |
| 51 | 448 | C | 0.0 | 0.0 | -21.8899 | -0.010612 | 0.008290534 | 0.008290534 | -0.01658107 |
| 52 | 450 | C | 1.3737 | 2.3793 | -17.9935 | -0.0010874 | -0.0354015 | 0.03091493 | 0.004486566 |
| 53 | 456 | C | 5.5059 | 9.5365 | -6.3246 | 0.021377 | -0.1335963 | 0.341155 | -0.2075587 |
| 54 | 462 | C | 6.8853 | 11.9257 | -2.4366 | -0.012353 | -0.1362827 | 0.2097366 | -0.07345394 |
| 55 | 468 | C | -1.3745 | -2.3806 | -14.095 | -0.0024334 | -0.03510775 | -0.08240255 | 0.1175103 |
| 56 | 474 | C | 6.8981 | 7.1656 | -2.433 | -0.045998 | -0.2062785 | 0.3837691 | -0.1774906 |
| 57 | 486 | C | 8.2695 | 9.5487 | 1.4581 | -0.10332 | -0.1397099 | 0.2108084 | -0.07109844 |
| 58 | 498 | C | 4.1493 | 7.1867 | 1.4601 | -0.98042 | -0.4026461 | 0.6313045 | -0.2286584 |
| 59 | 504 | C | 0.0 | 0.0 | -10.188 | 0.029617 | -0.181935 | -0.181935 | 0.3638699 |
| 60 | 506 | C | 5.5115 | 9.5463 | 5.352 | 0.024538 | -0.1267079 | 0.2802386 | -0.1535307 |

TABLE S5. Isotropic and anisotropic values for the hyperfine tensor with each lattice site for $^{13}C$ for the $SnV^0$ defect in diamond.

| Symmetry reduced # | Total # | Atom | x [Å] | y [Å] | z [Å] | Fermi [MHz] | $A_{xx}$ [MHz] | $A_{yy}$ [MHz] | $A_{zz}$ [MHz] |
|---|---|---|---|---|---|---|---|---|---|
| 1 | 1 | SN117 | 0.0 | 0.0 | 0.0 | 557.33 | 13.80647 | 13.80647 | -27.61293 |
| 1 | 1 | SN119 | 0.0 | 0.0 | 0.0 | 583.08 | 14.44428 | 14.44428 | -28.88856 |
| 2 | 2 | C | 1.3934 | 2.4134 | 5.3018 | -6.5473 | -0.5914604 | -0.2423933 | 0.8338537 |
| 3 | 8 | C | 2.7589 | 4.7785 | 9.2385 | 0.91215 | -0.1979265 | -0.2342727 | 0.4321992 |
| 4 | 14 | C | 4.129 | 7.1517 | 13.1322 | 0.10457 | -0.01510422 | -0.08683403 | 0.1019382 |
| 5 | 20 | C | -5.5047 | -9.5344 | -14.1079 | 0.055213 | 0.02628218 | -0.07897991 | 0.05269773 |
| 6 | 26 | C | -4.1321 | -7.1569 | -10.2171 | 0.61269 | -0.1046543 | 0.247031 | -0.1423767 |
| 7 | 32 | C | -2.7654 | -4.7899 | -6.3322 | 9.3407 | -1.128989 | 2.122665 | -0.9936764 |
| 8 | 38 | C | -1.555 | -2.6933 | -2.4597 | 63.941 | -13.16039 | 26.36026 | -13.19987 |
| 9 | 44 | C | -1.3747 | -2.3811 | 9.2068 | -0.36261 | -0.06913204 | -0.1279108 | 0.1970428 |
| 10 | 50 | C | 4.1232 | 2.3817 | 13.1214 | -0.011607 | -0.02137689 | -0.0561363 | 0.07751319 |
| 11 | 62 | C | -16.5191 | 4.7653 | 1.4544 | -0.013273 | 0.03102893 | -0.04634105 | 0.01531212 |
| 12 | 74 | C | -4.1358 | -11.9204 | -10.2173 | 0.028123 | 0.004362659 | 0.05337698 | -0.05773964 |
| 13 | 86 | C | -2.7586 | -9.5504 | -6.3282 | 0.44329 | -0.1222169 | 0.2713173 | -0.1491005 |
| 14 | 98 | C | -1.3811 | -7.2479 | -2.4342 | 7.6257 | -0.9975947 | 2.110799 | -1.113204 |
| 15 | 110 | C | 0.028 | -4.9033 | 1.4676 | -5.55 | -1.051305 | 1.229703 | -0.1783979 |
| 16 | 122 | C | 8.2605 | 14.3075 | 1.4531 | -0.0065143 | -0.03134926 | 0.03664078 | -0.005291511 |
| 17 | 128 | C | -15.1447 | 2.3817 | 5.349 | -0.016106 | 0.03669528 | -0.005883426 | -0.03081185 |
| 18 | 140 | C | -2.76 | -14.3076 | -6.3246 | 0.044169 | -0.005026036 | 0.05880389 | -0.05377785 |
| 19 | 152 | C | -1.3793 | -11.9546 | -2.4337 | 0.7736 | -0.1666485 | 0.3097766 | -0.1431281 |
| 20 | 164 | C | 0.0028 | -9.5985 | 1.4611 | 0.99721 | -0.3043854 | 0.5274739 | -0.2230885 |
| 21 | 176 | C | 1.3823 | -7.1797 | 5.3525 | -0.775 | -0.1461489 | 0.3302044 | -0.1840555 |
| 22 | 188 | C | 6.8837 | 11.9229 | 9.2431 | 0.0072128 | 0.006173298 | 0.03362052 | -0.03979381 |
| 23 | 194 | C | -1.3804 | -16.6926 | -2.4308 | 0.082898 | -0.06933615 | 0.06522427 | 0.004111875 |
| 24 | 206 | C | 0.0016 | -14.3227 | 1.4604 | 0.15304 | -0.09008189 | 0.1133497 | -0.02326781 |
| 25 | 218 | C | 1.3815 | -11.9326 | 5.3529 | -0.083313 | -0.07412991 | 0.1084751 | -0.03434515 |
| 26 | 230 | C | 2.7585 | -9.5408 | 9.244 | -0.081139 | -0.02164415 | 0.09988434 | -0.07824019 |
| 27 | 242 | C | -6.8852 | -11.9256 | -6.3238 | 0.18361 | -0.04425946 | 0.1032847 | -0.05902525 |
| 28 | 248 | C | 15.1487 | 2.3833 | -2.4288 | 0.037961 | 0.06359439 | -0.04763516 | -0.01595923 |
| 29 | 260 | C | -5.4973 | 4.7661 | -14.1008 | -0.011145 | 0.0533532 | -0.0598081 | 0.006454895 |
| 30 | 272 | C | 2.7477 | 4.7592 | -14.0988 | -0.013401 | -0.04915038 | -0.01650668 | 0.06565705 |
| 31 | 278 | C | -4.1259 | 2.3838 | -10.1988 | 0.0064325 | -0.09949692 | -0.06614756 | 0.1656445 |
| 32 | 290 | C | 1.3767 | 2.3845 | -6.2706 | 2.5569 | 0.3115702 | -0.6368724 | 0.3253022 |
| 33 | 296 | C | 0.0 | 0.0 | 13.1136 | -0.036117 | -0.0384545 | -0.0384545 | 0.07690899 |
| 34 | 298 | C | 1.3743 | 2.3803 | 17.017 | -0.010137 | 0.001518559 | -0.02206778 | 0.02054922 |
| 35 | 304 | C | -8.2584 | -14.304 | -10.2186 | 0.020318 | 0.007878295 | 0.01816753 | -0.02604583 |
| 36 | 310 | C | -5.5181 | -9.5576 | -2.431 | 0.52783 | -0.1505155 | 0.2977425 | -0.147227 |
| 37 | 316 | C | -4.1408 | -7.1721 | 1.4588 | -0.19879 | -0.1418486 | 0.2095373 | -0.06768869 |
| 38 | 322 | C | -2.7569 | -4.7751 | 5.3354 | -0.46117 | -0.1662337 | 0.4042299 | -0.2379961 |
| 39 | 328 | C | 9.6334 | 16.6855 | 5.3477 | 0.0063213 | -0.002478946 | 0.008443941 | -0.005964995 |
| 40 | 334 | C | -6.8846 | -16.6857 | -6.3231 | 0.0072179 | -0.001544387 | 0.02109146 | -0.01954707 |
| 41 | 346 | C | -4.1339 | -11.9319 | 1.462 | 0.0015566 | -0.07756539 | 0.1123459 | -0.03478055 |
| 42 | 358 | C | -2.7528 | -9.5424 | 5.3502 | -0.023592 | -0.08171363 | 0.1908279 | -0.1091143 |
| 43 | 370 | C | -1.3739 | -7.1505 | 9.2349 | -0.021171 | -0.07380299 | -0.1025978 | 0.1764008 |
| 44 | 382 | C | -2.7492 | -4.7617 | -17.9939 | -0.0049484 | 0.02088652 | -0.03482992 | 0.01394341 |
| 45 | 388 | C | 8.258 | 4.7611 | -10.2128 | 0.017886 | -0.08602433 | 0.1151217 | -0.0290974 |
| 46 | 400 | C | 9.6392 | 7.1499 | -6.3248 | 0.013474 | -0.04761707 | 0.1353068 | -0.08768978 |
| 47 | 412 | C | 11.0167 | 9.5393 | -2.4358 | -0.02173 | -0.07271505 | 0.08352148 | -0.01080642 |
| 48 | 424 | C | 4.1256 | 7.1458 | -10.2108 | 0.01827 | -0.06208534 | 0.1480059 | -0.08592056 |
| 49 | 430 | C | -6.8875 | 2.3882 | -6.318 | 0.30101 | 0.240591 | -0.02904017 | -0.2115508 |
| 50 | 442 | C | 2.7662 | 4.7912 | -2.4305 | 0.78572 | 0.1819578 | 0.2708393 | -0.4527971 |
| 51 | 448 | C | 0.0 | 0.0 | -21.8897 | -0.00025881 | 0.003301456 | 0.003301456 | -0.006602913 |
| 52 | 450 | C | 1.3736 | 2.3792 | -17.9928 | -0.00024773 | -0.01745702 | 0.01520085 | 0.002256171 |
| 53 | 456 | C | 5.5058 | 9.5363 | -6.3245 | 0.0034044 | -0.06933983 | 0.1728657 | -0.1035259 |
| 54 | 462 | C | 6.8855 | 11.926 | -2.4371 | -0.0083478 | -0.06842869 | 0.1058658 | -0.03743716 |
| 55 | 468 | C | -1.3743 | -2.3804 | -14.0938 | -0.017688 | -0.01774041 | -0.04164044 | 0.05938085 |
| 56 | 474 | C | 6.8981 | 7.1653 | -2.4327 | -0.055355 | -0.1046943 | 0.1954752 | -0.09078088 |
| 57 | 486 | C | 8.27 | 9.5493 | 1.4579 | -0.11355 | -0.06970359 | 0.1048835 | -0.03517987 |
| 58 | 498 | C | 4.1497 | 7.1876 | 1.4593 | -1.0184 | -0.203265 | 0.3184428 | -0.1151778 |
| 59 | 504 | C | 0.0 | 0.0 | -10.1852 | 0.043106 | -0.09222582 | -0.09222582 | 0.1844516 |
| 60 | 506 | C | 5.5116 | 9.5464 | 5.3515 | 0.0073224 | -0.06226198 | 0.1377975 | -0.07553551 |

TABLE S6. Isotropic and anisotropic values for the hyperfine tensor with each lattice site for $^{13}C$ for the $SnV^-$ defect in diamond.

| Symmetry reduced # | Total # | Atom | x [Å] | y [Å] | z [Å] | $R_{xx}$ | $R_{xy}$ | $R_{xz}$ | $R_{yx}$ | $R_{yy}$ | $R_{yz}$ | $R_{zx}$ | $R_{zy}$ | $R_{zz}$ |
|---|---|---|---|---|---|---|---|---|---|---|---|---|---|---|
| 1 | 1 | SI | 0.0 | 0.0 | 0.0 | 1.0 | 0.0 | 0.0 | 0.0 | 1.0 | 0.0 | 0.0 | 0.0 | 1.0 |
| 2 | 2 | C | 1.3732 | 2.3784 | 5.2584 | 0.8660254 | -0.5 | 0.0 | 0.3742569 | 0.648232 | 0.6631192 | -0.3315596 | -0.5742781 | 0.7485138 |
| 3 | 8 | C | 2.7508 | 4.7646 | 9.219 | 0.8660254 | -0.5 | 3.164559e-13 | 0.4406344 | 0.7632011 | -0.4726155 | 0.2363077 | 0.409297 | 0.8812688 |
| 4 | 14 | C | 4.1269 | 7.1479 | 13.1266 | 0.8660254 | -0.5 | -2.242819e-09 | 0.4385927 | 0.7596649 | -0.4801517 | 0.2400759 | 0.4158236 | 0.8771855 |
| 5 | 20 | C | -5.5039 | -9.533 | -14.1062 | 0.8660254 | -0.5 | 0.0 | 0.4133716 | 0.7159805 | -0.5625796 | 0.2812898 | 0.4872082 | 0.8267431 |
| 6 | 26 | C | -4.1281 | -7.1501 | -10.2053 | 0.8660254 | -0.5 | 0.0 | 0.3944613 | 0.683227 | 0.6144926 | -0.3072463 | -0.5321662 | 0.7889226 |
| 7 | 32 | C | -2.7558 | -4.7731 | -6.2948 | 0.8660254 | -0.5 | 0.0 | 0.4531307 | 0.7848455 | 0.4227175 | -0.2113588 | -0.3660841 | 0.9062615 |
| 8 | 38 | C | -1.476 | -2.5566 | -2.3459 | 0.8660254 | -0.5 | 0.0 | 0.4746653 | 0.8221444 | 0.3142794 | -0.1571397 | -0.2721739 | 0.9493305 |
| 9 | 44 | C | -1.3731 | -2.3783 | 9.1993 | 0.8660254 | -0.5 | -8.051803e-14 | 0.467513 | 0.8097563 | 0.354579 | -0.1772895 | -0.3070744 | 0.9350261 |
| 10 | 50 | C | 4.1228 | 2.3812 | 13.1173 | 0.8145086 | -0.4632953 | -0.3491894 | 0.3562589 | 0.8744671 | -0.3292215 | 0.4578814 | 0.143752 | 0.8773141 |
| 11 | 62 | C | -16.517 | 4.7654 | 1.4533 | 0.9532148 | -0.2770999 | 0.1208188 | 0.297323 | 0.7872224 | -0.5402592 | 0.05459452 | 0.5509052 | 0.8327802 |
| 12 | 74 | C | -4.1329 | -11.9182 | -10.2161 | 0.9500937 | -0.2999147 | -0.0858668 | 0.2868126 | 0.7314771 | 0.6186112 | -0.122721 | -0.6123663 | 0.7809911 |
| 13 | 86 | C | -2.7566 | -9.5435 | -6.324 | 0.888168 | -0.2293828 | -0.3981723 | 0.3956913 | 0.8223334 | 0.4088962 | 0.2336366 | -0.5207218 | 0.821135 |
| 14 | 98 | C | -1.3833 | -7.2116 | -2.4343 | 0.7380888 | -0.4750587 | 0.4791076 | 0.3826913 | 0.8795921 | 0.282604 | -0.5556728 | -0.02523657 | 0.831018 |
| 15 | 110 | C | 0.0112 | -4.8589 | 1.4465 | 0.8658224 | 0.065419 | -0.4960563 | 0.0134782 | 0.9880067 | 0.1538215 | 0.5001698 | -0.1398681 | 0.8545566 |
| 16 | 122 | C | 8.2592 | 14.3054 | 1.4515 | 0.8660254 | -0.5 | 0.0 | 0.4889082 | 0.8468138 | -0.2094639 | 0.104732 | 0.1814011 | 0.9778164 |
| 17 | 128 | C | -15.1418 | 2.3823 | 5.3486 | 0.9508874 | -0.1665363 | -0.2609194 | 0.274753 | 0.8423305 | 0.4636702 | 0.1425624 | -0.5125865 | 0.8467178 |
| 18 | 140 | C | -2.757 | -14.3046 | -6.3242 | 0.8904068 | -0.01531044 | -0.454908 | 0.2046518 | 0.9061807 | 0.3700733 | 0.4065628 | -0.4226135 | 0.8100028 |
| 19 | 152 | C | -1.3787 | -11.9397 | -2.4328 | 0.6303195 | -0.3605692 | 0.6875225 | 0.2815339 | 0.9314793 | 0.2304019 | -0.7234888 | 0.04833409 | 0.688642 |
| 20 | 164 | C | 0.0007 | -9.5726 | 1.4589 | 0.9741447 | -0.09245686 | -0.2061402 | 0.1162014 | 0.9875312 | 0.1062044 | 0.1937506 | -0.1274122 | 0.9727419 |
| 21 | 176 | C | 1.3793 | -7.1671 | 5.344 | 0.6498573 | 0.5073853 | 0.5659025 | -0.176773 | 0.8250335 | -0.5367225 | -0.7392136 | 0.2487567 | 0.6258461 |
| 22 | 188 | C | 6.8823 | 11.9205 | 9.2429 | 0.8660254 | -0.5 | 3.508266e-09 | 0.4052397 | 0.7018957 | 0.5857672 | -0.2928836 | -0.5072892 | 0.8104794 |
| 23 | 194 | C | -1.3788 | -16.6887 | -2.4312 | 0.7814028 | -0.142094 | 0.6076339 | 0.09631319 | 0.9895244 | 0.1075419 | -0.6165496 | -0.02551038 | 0.7869026 |
| 24 | 206 | C | 0.0004 | -14.3137 | 1.4601 | 0.8757545 | -0.07033421 | 0.4776057 | 0.06345483 | 0.9975171 | 0.03054555 | -0.4785683 | 0.00355599 | 0.8780431 |
| 25 | 218 | C | 1.3792 | -11.926 | 5.3512 | 0.8266536 | -0.2121574 | -0.5211843 | -0.02847884 | 0.9092416 | -0.4152935 | 0.56199 | 0.3581466 | 0.7455858 |
| 26 | 230 | C | 2.7556 | -9.5364 | 9.2399 | 0.966287 | 0.2442242 | 0.08151035 | -0.1232732 | 0.7167924 | -0.6863034 | -0.2260379 | 0.653118 | 0.7227335 |
| 27 | 242 | C | -6.8836 | -11.9228 | -6.3232 | 0.8660254 | -0.5 | 0.0 | 0.4671984 | 0.8092114 | 0.3562337 | -0.1781169 | -0.3085075 | 0.9343969 |
| 28 | 248 | C | 15.145 | 2.3832 | -2.428 | 0.9769883 | 0.1471791 | -0.1543767 | -0.06780073 | 0.9005349 | 0.4294647 | 0.2022299 | -0.4091152 | 0.8897909 |
| 29 | 260 | C | -5.4982 | 4.7651 | -14.0981 | 0.6870045 | -0.08100161 | 0.7221243 | -0.394472 | 0.7930147 | 0.4642407 | -0.6102595 | -0.6037933 | 0.5128518 |
| 30 | 272 | C | 2.7483 | 4.7602 | -14.0956 | 0.8660254 | -0.5 | 0.0 | 0.3612203 | 0.6256518 | -0.6914331 | 0.3457165 | 0.5987986 | 0.7224405 |
| 31 | 278 | C | -4.1238 | 2.3812 | -10.1912 | 0.8030931 | -0.3794588 | -0.4594045 | 0.4100483 | 0.9113551 | -0.03594816 | 0.4323214 | -0.1595083 | 0.8874995 |
| 32 | 290 | C | 1.3743 | 2.3804 | -6.258 | 0.8660254 | -0.5 | 0.0 | 0.444374 | 0.7696783 | 0.4583962 | -0.2291981 | -0.3969828 | 0.8887479 |
| 33 | 296 | C | 0.0 | 0.0 | 13.1111 | 1.0 | 0.0 | 0.0 | 0.0 | 1.0 | 0.0 | 0.0 | 0.0 | 1.0 |
| 34 | 298 | C | 1.3746 | 2.3809 | 17.0157 | 0.8660254 | -0.5 | 0.0 | 0.458837 | 0.794729 | -0.3973341 | 0.1986671 | 0.3441014 | 0.917674 |
| 35 | 304 | C | -8.2576 | -14.3026 | -10.2188 | 0.8660254 | -0.5 | 1.298404e-10 | 0.434977 | 0.7534023 | 0.4931328 | -0.2465664 | -0.4270656 | 0.869954 |
| 36 | 310 | C | -5.514 | -9.5506 | -2.431 | 0.8660254 | -0.5 | 0.0 | 0.4792686 | 0.8301175 | 0.2849676 | -0.1424838 | -0.2467892 | 0.9585371 |
| 37 | 316 | C | -4.1383 | -7.1678 | 1.4571 | 0.8660254 | -0.5 | 0.0 | 0.4983376 | 0.863146 | -0.08147735 | 0.04073867 | 0.07056145 | 0.9966752 |
| 38 | 322 | C | -2.7555 | -4.7727 | 5.3305 | 0.8660254 | -0.5 | 0.0 | 0.3633161 | 0.629282 | 0.6870266 | -0.3435133 | -0.5949825 | 0.7266323 |
| 39 | 328 | C | 9.6329 | 16.6846 | 5.3472 | 0.8660254 | -0.5 | 0.0 | 0.4999696 | 0.8659728 | -0.01102509 | 0.005512545 | 0.009548007 | 0.9999392 |
| 40 | 334 | C | -6.8832 | -16.6848 | -6.3229 | 0.9011776 | -0.2749186 | -0.33511 | 0.3459054 | 0.9220345 | 0.1737867 | 0.2612058 | -0.272529 | 0.9260127 |
| 41 | 346 | C | -4.1326 | -11.9278 | 1.4625 | 0.9102998 | -0.2715442 | 0.3124388 | 0.3498603 | 0.9081082 | -0.2300812 | -0.221251 | 0.3187528 | 0.9216532 |
| 42 | 358 | C | -2.7529 | -9.5397 | 5.3492 | 0.6833813 | -0.6126361 | -0.397073 | 0.3403208 | 0.7485036 | -0.5691433 | 0.6458884 | 0.2538097 | 0.7200061 |
| 43 | 370 | C | -1.3746 | -7.1489 | 9.232 | 0.9581332 | -0.05106222 | 0.281733 | -0.135702 | 0.7854533 | 0.603861 | -0.2521226 | -0.616811 | 0.7456396 |
| 44 | 382 | C | -2.7498 | -4.7628 | -17.9932 | 0.8660254 | -0.5 | 0.0 | 0.4129231 | 0.7152039 | -0.5638953 | 0.2819476 | 0.4883476 | 0.8258463 |
| 45 | 388 | C | 8.2562 | 4.7624 | -10.2111 | 0.6784343 | 0.2270465 | 0.6986965 | 0.4852447 | 0.5755818 | -0.6582121 | -0.5516018 | 0.7855924 | 0.2803213 |
| 46 | 400 | C | 9.6366 | 7.1502 | -6.3247 | 0.831494 | -0.522132 | 0.1897256 | 0.5256888 | 0.6290829 | -0.5726308 | 0.1796357 | 0.5758757 | 0.7975576 |
| 47 | 412 | C | 11.0137 | 9.538 | -2.4368 | 0.4856502 | -0.7002679 | -0.5232291 | 0.5030343 | 0.7133968 | -0.4878745 | 0.7149128 | -0.02626586 | 0.6987201 |
| 48 | 424 | C | 4.1258 | 7.1462 | -10.209 | 0.8660254 | -0.5 | 0.0 | 0.3751048 | 0.6497006 | -0.6612 | 0.3306 | 0.572616 | 0.7502097 |
| 49 | 430 | C | -6.8845 | 2.3861 | -6.3145 | 0.7011631 | -0.3423906 | 0.625411 | 0.2617591 | 0.9395162 | 0.2208878 | -0.6632137 | 0.008828608 | 0.748378 |
| 50 | 442 | C | 2.7635 | 4.7865 | -2.4232 | 0.8660254 | -0.5 | 0.0 | 0.4640827 | 0.8038148 | -0.3721681 | 0.186084 | 0.322307 | 0.9281654 |
| 51 | 448 | C | -0.0 | 0.0 | -21.8894 | 1.0 | 0.0 | 0.0 | 0.0 | 1.0 | 0.0 | 0.0 | 0.0 | 1.0 |
| 52 | 450 | C | 1.3742 | 2.3802 | -17.9918 | 0.8660254 | -0.5 | 0.0 | 0.4942558 | 0.8560762 | -0.1511444 | 0.0755722 | 0.1308949 | 0.9885117 |
| 53 | 456 | C | 5.5053 | 9.5355 | -6.3246 | 0.8660254 | -0.5 | 0.0 | 0.4022339 | 0.6966896 | -0.5939962 | 0.2969981 | 0.5144158 | 0.8044678 |
| 54 | 462 | C | 6.8841 | 11.9236 | -2.4386 | 0.8660254 | -0.5 | 0.0 | 0.4242421 | 0.7348089 | -0.5292206 | 0.2646103 | 0.4583185 | 0.8484842 |
| 55 | 468 | C | -1.3744 | -2.3805 | -14.0913 | 0.8660254 | -0.5 | 0.0 | 0.4854368 | 0.8408012 | -0.2395923 | 0.1197961 | 0.207493 | 0.9708736 |
| 56 | 474 | C | 6.8925 | 7.1611 | -2.4321 | 0.7405341 | -0.350565 | 0.5733354 | 0.5956044 | 0.7374998 | -0.3183543 | -0.3112308 | 0.5772333 | 0.7549418 |
| 57 | 486 | C | 8.2653 | 9.544 | 1.457 | 0.7016222 | -0.5673019 | -0.4311552 | 0.6622364 | 0.7424966 | 0.1007063 | 0.2630005 | -0.3561844 | 0.8966401 |
| 58 | 498 | C | 4.1424 | 7.1749 | 1.4595 | 0.8660254 | -0.5 | 0.0 | 0.4873904 | 0.844185 | 0.2231641 | -0.111582 | -0.1932658 | 0.9747809 |
| 59 | 504 | C | 0.0 | 0.0 | -10.1807 | 1.0 | 0.0 | 0.0 | 0.0 | 1.0 | 0.0 | 0.0 | 0.0 | 1.0 |
| 60 | 506 | C | 5.509 | 9.5419 | 5.3499 | 0.8660254 | -0.5 | 0.0 | 0.4520012 | 0.782889 | 0.4275276 | -0.2137638 | -0.3702497 | 0.9040023 |

TABLE S7. Elements of rotation matrix from Cartesian to principal axes of hyperfine tensor with each lattice site for $^{13}C$ for the $SiV^0$ defect in diamond.

| Symmetry reduced # | Total # | Atom | x [Å] | y [Å] | z [Å] | $R_{xx}$ | $R_{xy}$ | $R_{xz}$ | $R_{yx}$ | $R_{yy}$ | $R_{yz}$ | $R_{zx}$ | $R_{zy}$ | $R_{zz}$ |
|---|---|---|---|---|---|---|---|---|---|---|---|---|---|---|
| 1 | 1 | SI | 0.0 | 0.0 | 0.0 | 1.0 | 0.0 | 0.0 | 0.0 | 1.0 | 0.0 | 0.0 | 0.0 | 1.0 |
| 2 | 2 | C | 1.3735 | 2.3789 | 5.243 | 0.8660254 | -0.5 | 0.0 | 0.3571402 | 0.618585 | 0.6998595 | -0.3499298 | -0.6060961 | 0.7142805 |
| 3 | 8 | C | 2.751 | 4.7648 | 9.2154 | 0.8660254 | -0.5 | 6.361809e-13 | 0.4410008 | 0.7638357 | -0.4712465 | 0.2356233 | 0.4081115 | 0.8820015 |
| 4 | 14 | C | 4.1268 | 7.1479 | 13.1258 | 0.8660254 | -0.5 | -3.193269e-09 | 0.4379923 | 0.7586249 | -0.4823391 | 0.2411695 | 0.4177179 | 0.8759846 |
| 5 | 20 | C | -5.5039 | -9.533 | -14.1061 | 0.8660254 | -0.5 | 0.0 | 0.4132212 | 0.7157201 | -0.5630212 | 0.2815106 | 0.4875907 | 0.8264424 |
| 6 | 26 | C | -4.1277 | -7.1493 | -10.2045 | 0.8660254 | -0.5 | 0.0 | 0.3914672 | 0.678041 | 0.6221043 | -0.3110522 | -0.5387582 | 0.7829343 |
| 7 | 32 | C | -2.7532 | -4.7687 | -6.2914 | 0.8660254 | -0.5 | 0.0 | 0.4519157 | 0.782741 | 0.4278886 | -0.2139443 | -0.3705624 | 0.9038315 |
| 8 | 38 | C | -1.4653 | -2.538 | -2.3252 | 0.8660254 | -0.5 | 0.0 | 0.4737362 | 0.8205352 | 0.3198373 | -0.1599186 | -0.2769872 | 0.9474725 |
| 9 | 44 | C | -1.3727 | -2.3775 | 9.1929 | 0.8660254 | -0.5 | -2.58856e-13 | 0.4678454 | 0.810332 | 0.352821 | -0.1764105 | -0.305552 | 0.9356908 |
| 10 | 50 | C | 4.1225 | 2.381 | 13.1151 | 0.815438 | -0.4588884 | -0.3528205 | 0.3524506 | 0.8771265 | -0.3262326 | 0.4591725 | 0.1416707 | 0.8769778 |
| 11 | 62 | C | -16.5172 | 4.7653 | 1.4526 | 0.9530447 | -0.2673391 | 0.1422518 | 0.3012566 | 0.7891652 | -0.5352222 | 0.03082569 | 0.552945 | 0.8326474 |
| 12 | 74 | C | -4.1329 | -11.918 | -10.2161 | 0.9570815 | -0.282584 | -0.06435262 | 0.2590108 | 0.7343661 | 0.6273913 | -0.1300324 | -0.6171326 | 0.7760405 |
| 13 | 86 | C | -2.756 | -9.5424 | -6.3233 | 0.8927955 | -0.2245033 | -0.390531 | 0.3884411 | 0.8226924 | 0.4150791 | 0.2281003 | -0.522279 | 0.8217024 |
| 14 | 98 | C | -1.3801 | -7.212 | -2.4313 | 0.7396772 | -0.4761471 | 0.4755645 | 0.3817304 | 0.8788485 | 0.2861944 | -0.5542198 | -0.03015408 | 0.831824 |
| 15 | 110 | C | 0.0203 | -4.8584 | 1.4497 | 0.8741701 | 0.04735184 | -0.4833057 | 0.03277319 | 0.9872132 | 0.156 | 0.4845127 | -0.15221 | 0.8614404 |
| 16 | 122 | C | 8.2594 | 14.3056 | 1.4505 | 0.8660254 | -0.5 | 0.0 | 0.4861996 | 0.8421224 | -0.2333232 | 0.1166616 | 0.2020639 | 0.9723992 |
| 17 | 128 | C | -15.1418 | 2.3822 | 5.3483 | 0.9455201 | -0.1803966 | -0.2710145 | 0.2950484 | 0.8266866 | 0.4790988 | 0.1376162 | -0.5329599 | 0.8348745 |
| 18 | 140 | C | -2.7569 | -14.3046 | -6.3241 | 0.8941334 | 0.0192705 | -0.4473858 | 0.1731604 | 0.906476 | 0.385119 | 0.4129659 | -0.4218173 | 0.8071737 |
| 19 | 152 | C | -1.3781 | -11.9411 | -2.4323 | 0.6433329 | -0.3586556 | 0.6763793 | 0.2763151 | 0.9327045 | 0.2317592 | -0.7139837 | 0.03779549 | 0.6991414 |
| 20 | 164 | C | 0.0021 | -9.5747 | 1.4595 | 0.9772874 | -0.09442294 | -0.1897199 | 0.114561 | 0.9885581 | 0.09812599 | 0.1782838 | -0.1176318 | 0.9769225 |
| 21 | 176 | C | 1.3798 | -7.1666 | 5.3421 | 0.6562035 | 0.5075908 | 0.5583445 | -0.1667597 | 0.819192 | -0.54874 | -0.7359268 | 0.2669757 | 0.6222024 |
| 22 | 188 | C | 6.8823 | 11.9205 | 9.2427 | 0.8660254 | -0.5 | 6.152069e-09 | 0.401004 | 0.6945593 | 0.5973134 | -0.2986567 | -0.5172886 | 0.8020079 |
| 23 | 194 | C | -1.3788 | -16.6893 | -2.431 | 0.7827703 | -0.1375566 | 0.6069174 | 0.08902207 | 0.9899855 | 0.1095621 | -0.6159104 | -0.03173291 | 0.7871768 |
| 24 | 206 | C | 0.0007 | -14.3149 | 1.4603 | 0.8719047 | -0.06637423 | 0.4851563 | 0.06495834 | 0.9976924 | 0.0197536 | -0.4853479 | 0.01429169 | 0.8742043 |
| 25 | 218 | C | 1.3792 | -11.9262 | 5.3511 | 0.8272813 | -0.2300008 | -0.5125479 | -0.01154724 | 0.9051967 | -0.4248359 | 0.5616692 | 0.3573773 | 0.7461964 |
| 26 | 230 | C | 2.7556 | -9.5363 | 9.2393 | 0.9653012 | 0.2418011 | 0.09861912 | -0.1090953 | 0.7165239 | -0.6889788 | -0.2372588 | 0.6543132 | 0.7180407 |
| 27 | 242 | C | -6.8834 | -11.9225 | -6.3228 | 0.8660254 | -0.5 | 0.0 | 0.4660779 | 0.8072707 | 0.3620572 | -0.1810286 | -0.3135508 | 0.9321559 |
| 28 | 248 | C | 15.145 | 2.3832 | -2.4273 | 0.9777902 | 0.1492823 | -0.1471092 | -0.07395701 | 0.9025097 | 0.4242718 | 0.1961037 | -0.403969 | 0.8935057 |
| 29 | 260 | C | -5.4979 | 4.7648 | -14.0971 | 0.6825673 | -0.08765221 | 0.7255473 | -0.3930767 | 0.7929206 | 0.4655831 | -0.6161108 | -0.6029876 | 0.5067676 |
| 30 | 272 | C | 2.7482 | 4.76 | -14.0943 | 0.8660254 | -0.5 | 0.0 | 0.3596245 | 0.6228879 | -0.6947524 | 0.3473762 | 0.6016732 | 0.719249 |
| 31 | 278 | C | -4.1228 | 2.3807 | -10.1884 | 0.7860552 | -0.4148702 | -0.4582575 | 0.440681 | 0.8959632 | -0.05522841 | 0.4334944 | -0.1585328 | 0.887102 |
| 32 | 290 | C | 1.372 | 2.3764 | -6.2499 | 0.8660254 | -0.5 | 0.0 | 0.4449135 | 0.7706129 | 0.4562979 | -0.2281489 | -0.3951655 | 0.8898271 |
| 33 | 296 | C | 0.0 | 0.0 | 13.1078 | 1.0 | 0.0 | 0.0 | 0.0 | 1.0 | 0.0 | 0.0 | 0.0 | 1.0 |
| 34 | 298 | C | 1.3745 | 2.3808 | 17.0144 | 0.8660254 | -0.5 | 0.0 | 0.4636523 | 0.8030693 | -0.3743077 | 0.1871538 | 0.32416 | 0.9273046 |
| 35 | 304 | C | -8.2576 | -14.3026 | -10.2191 | 0.8660254 | -0.5 | 1.999344e-10 | 0.4281845 | 0.7416374 | 0.5163642 | -0.2581821 | -0.4471845 | 0.8563691 |
| 36 | 310 | C | -5.5136 | -9.5498 | -2.43 | 0.8660254 | -0.5 | 0.0 | 0.4795434 | 0.8305936 | 0.2831121 | -0.141556 | -0.2451823 | 0.9590868 |
| 37 | 316 | C | -4.1365 | -7.1646 | 1.457 | 0.8660254 | -0.5 | 0.0 | 0.4975382 | 0.8617614 | -0.09911092 | 0.04955546 | 0.08583258 | 0.9950764 |
| 38 | 322 | C | -2.7541 | -4.7703 | 5.3267 | 0.8660254 | -0.5 | 0.0 | 0.3641082 | 0.6306539 | 0.6853473 | -0.3426737 | -0.5935282 | 0.7282163 |
| 39 | 328 | C | 9.6329 | 16.6847 | 5.3468 | 0.8660254 | -0.5 | 0.0 | 0.4999278 | 0.8659004 | -0.01699292 | 0.008496461 | 0.0147163 | 0.9998556 |
| 40 | 334 | C | -6.8832 | -16.6847 | -6.3227 | 0.8953832 | -0.2517595 | -0.3672955 | 0.3350552 | 0.9241951 | 0.1833072 | 0.2933034 | -0.2871944 | 0.9118621 |
| 41 | 346 | C | -4.1324 | -11.9274 | 1.463 | 0.9096814 | -0.2710409 | 0.3146691 | 0.3530345 | 0.9037271 | -0.2421652 | -0.2187383 | 0.3313822 | 0.9177905 |
| 42 | 358 | C | -2.7526 | -9.5388 | 5.3487 | 0.6802467 | -0.61098 | -0.4049295 | 0.3391886 | 0.7521215 | -0.5650348 | 0.6497811 | 0.2470156 | 0.7188656 |
| 43 | 370 | C | -1.3745 | -7.1483 | 9.2302 | 0.9516465 | -0.01622579 | 0.3067664 | -0.1773123 | 0.7864518 | 0.5916536 | -0.250857 | -0.6174386 | 0.745547 |
| 44 | 382 | C | -2.7497 | -4.7626 | -17.9925 | 0.8660254 | -0.5 | 0.0 | 0.4163488 | 0.7211372 | -0.5537281 | 0.276864 | 0.4795426 | 0.8326976 |
| 45 | 388 | C | 8.2557 | 4.7623 | -10.2105 | 0.686402 | 0.2147899 | 0.6947788 | 0.4824974 | 0.5803055 | -0.6560807 | -0.5441034 | 0.785564 | 0.2946873 |
| 46 | 400 | C | 9.6362 | 7.1502 | -6.3247 | 0.8356376 | -0.5138819 | 0.1939981 | 0.5220734 | 0.6332794 | -0.5713113 | 0.1707315 | 0.5786905 | 0.7974761 |
| 47 | 412 | C | 11.0137 | 9.5382 | -2.4373 | 0.4845849 | -0.7009132 | -0.5233528 | 0.5006907 | 0.7128405 | -0.4910879 | 0.7172771 | -0.02406407 | 0.6963724 |
| 48 | 424 | C | 4.1257 | 7.1459 | -10.2081 | 0.8660254 | -0.5 | 0.0 | 0.3761592 | 0.6515268 | -0.6587998 | 0.3293999 | 0.5705373 | 0.7523183 |
| 49 | 430 | C | -6.8828 | 2.3855 | -6.3128 | 0.7072588 | -0.3226809 | 0.6290167 | 0.2491568 | 0.9464382 | 0.2053669 | -0.6615935 | 0.0114763 | 0.7497749 |
| 50 | 442 | C | 2.7606 | 4.7816 | -2.421 | 0.8660254 | -0.5 | -1.231559e-12 | 0.4637095 | 0.8031684 | -0.3740242 | 0.1870121 | 0.3239144 | 0.927419 |
| 51 | 448 | C | -0.0 | 0.0 | -21.8892 | 1.0 | 0.0 | 0.0 | 0.0 | 1.0 | 0.0 | 0.0 | 0.0 | 1.0 |
| 52 | 450 | C | 1.3741 | 2.3801 | -17.9909 | 0.8660254 | -0.5 | 0.0 | 0.4902422 | 0.8491243 | -0.1965973 | 0.09829864 | 0.1702582 | 0.9804843 |
| 53 | 456 | C | 5.5052 | 9.5352 | -6.3246 | 0.8660254 | -0.5 | 0.0 | 0.4033396 | 0.6986046 | -0.5909896 | 0.2954948 | 0.511812 | 0.8066791 |
| 54 | 462 | C | 6.8841 | 11.9237 | -2.4393 | 0.8660254 | -0.5 | 0.0 | 0.4243118 | 0.7349295 | -0.5289973 | 0.2644987 | 0.4581251 | 0.8486235 |
| 55 | 468 | C | -1.3742 | -2.3802 | -14.0894 | 0.8660254 | -0.5 | 0.0 | 0.4854733 | 0.8408644 | -0.2392965 | 0.1196482 | 0.2072368 | 0.9709466 |
| 56 | 474 | C | 6.8919 | 7.1605 | -2.4316 | 0.7357421 | -0.3426593 | 0.5841816 | 0.5965566 | 0.7362451 | -0.3194735 | -0.3206303 | 0.5835475 | 0.7461022 |
| 57 | 486 | C | 8.2655 | 9.5443 | 1.4568 | 0.6997736 | -0.5698553 | -0.430792 | 0.6619026 | 0.7440519 | 0.09094877 | 0.268704 | -0.3487859 | 0.8978567 |
| 58 | 498 | C | 4.1425 | 7.175 | 1.4593 | 0.8660254 | -0.5 | 0.0 | 0.4883455 | 0.8458392 | 0.21465 | -0.107325 | -0.1858924 | 0.976691 |
| 59 | 504 | C | -0.0 | 0.0 | -10.1765 | 1.0 | 0.0 | 0.0 | 0.0 | 1.0 | 0.0 | 0.0 | 0.0 | 1.0 |
| 60 | 506 | C | 5.5089 | 9.5417 | 5.3494 | 0.8660254 | -0.5 | 0.0 | 0.4509752 | 0.7811119 | 0.4318397 | -0.2159198 | -0.3739841 | 0.9019504 |

TABLE S8. Elements of rotation matrix from Cartesian to principal axes of hyperfine tensor with each lattice site for $^{13}C$ for the $SiV^{-}$ defect in diamond.

| Symmetry reduced # | Total # | Atom | x [Å] | y [Å] | z [Å] | $R_{xx}$ | $R_{xy}$ | $R_{xz}$ | $R_{yx}$ | $R_{yy}$ | $R_{yz}$ | $R_{zx}$ | $R_{zy}$ | $R_{zz}$ |
|---|---|---|---|---|---|---|---|---|---|---|---|---|---|---|
| 1 | 1 | GE | 0.0 | 0.0 | 0.0 | 1.0 | 0.0 | 0.0 | 0.0 | 1.0 | 0.0 | 0.0 | 0.0 | 1.0 |
| 2 | 2 | C | 1.3777 | 2.3862 | 5.271 | 0.8660254 | -0.5 | 0.0 | 0.3556058 | 0.6159273 | -0.702978 | 0.351489 | 0.6087968 | 0.7112116 |
| 3 | 8 | C | 2.7526 | 4.7676 | 9.2235 | 0.8660254 | -0.5 | 4.772066e-13 | 0.4526005 | 0.7839271 | -0.4249836 | 0.2124918 | 0.3680466 | 0.905201 |
| 4 | 14 | C | 4.1273 | 7.1488 | 13.1278 | 0.8660254 | -0.5 | -1.027738e-09 | 0.4431253 | 0.7675156 | -0.463206 | 0.231603 | 0.4011481 | 0.8862507 |
| 5 | 20 | C | -5.5041 | -9.5334 | -14.1065 | 0.8660254 | -0.5 | 0.0 | 0.4133651 | 0.7159693 | -0.5625986 | 0.2812993 | 0.4872247 | 0.8267302 |
| 6 | 26 | C | -4.1291 | -7.1518 | -10.2077 | 0.8660254 | -0.5 | 0.0 | 0.3921193 | 0.6791706 | 0.6204593 | -0.3102297 | -0.5373335 | 0.7842386 |
| 7 | 32 | C | -2.7588 | -4.7783 | -6.3028 | 0.8660254 | -0.5 | 0.0 | 0.4504829 | 0.7802592 | 0.4338903 | -0.2169451 | -0.37576 | 0.9009657 |
| 8 | 38 | C | -1.5017 | -2.601 | -2.3766 | 0.8660254 | -0.5 | 0.0 | 0.4733237 | 0.8198208 | 0.3222709 | -0.1611354 | -0.2790948 | 0.9466475 |
| 9 | 44 | C | -1.3735 | -2.379 | 9.2018 | 0.8660254 | -0.5 | -1.220185e-14 | 0.4652662 | 0.8058648 | 0.3662094 | -0.1831047 | -0.3171466 | 0.9305325 |
| 10 | 50 | C | 4.1229 | 2.3814 | 13.1184 | 0.8076881 | -0.4699715 | -0.3560432 | 0.3640763 | 0.8725241 | -0.325807 | 0.4637763 | 0.1335235 | 0.8758328 |
| 11 | 62 | C | -16.5175 | 4.7654 | 1.4535 | 0.9496194 | -0.2374397 | 0.2045614 | 0.3112535 | 0.7908592 | -0.5269374 | -0.03666342 | 0.5640604 | 0.8249191 |
| 12 | 74 | C | -4.1337 | -11.9189 | -10.2165 | 0.9708964 | -0.2394882 | -0.002347432 | 0.1845831 | 0.7419912 | 0.6444984 | -0.152608 | -0.6261745 | 0.7646021 |
| 13 | 86 | C | -2.7573 | -9.5457 | -6.3251 | 0.9101465 | -0.2205972 | -0.3506711 | 0.3654825 | 0.8261138 | 0.4289038 | 0.1950793 | -0.5185295 | 0.832509 |
| 14 | 98 | C | -1.3835 | -7.2216 | -2.4347 | 0.7095488 | -0.4736196 | 0.5217518 | 0.3766918 | 0.8806999 | 0.2871777 | -0.5955197 | -0.007226954 | 0.8033082 |
| 15 | 110 | C | 0.014 | -4.8722 | 1.4509 | 0.893391 | 0.07501412 | -0.4429734 | 0.01500355 | 0.9804316 | 0.1962877 | 0.4490295 | -0.1820079 | 0.8747832 |
| 16 | 122 | C | 8.2596 | 14.3061 | 1.4518 | 0.8660254 | -0.5 | 0.0 | 0.4790506 | 0.8297399 | -0.2864301 | 0.143215 | 0.2480557 | 0.9581012 |
| 17 | 128 | C | -15.1427 | 2.3821 | 5.3487 | 0.9340362 | -0.2127028 | -0.2869388 | 0.3361385 | 0.7951094 | 0.504789 | 0.1207777 | -0.5679424 | 0.8141586 |
| 18 | 140 | C | -2.7578 | -14.3055 | -6.3243 | 0.8998404 | 0.1010301 | -0.4243586 | 0.09611657 | 0.9029812 | 0.4187917 | 0.4254984 | -0.4176336 | 0.8028283 |
| 19 | 152 | C | -1.3791 | -11.9435 | -2.433 | 0.6702137 | -0.3579818 | 0.6501251 | 0.2706875 | 0.9335455 | 0.2349914 | -0.6910441 | 0.0184863 | 0.7225762 |
| 20 | 164 | C | 0.0011 | -9.5793 | 1.4594 | 0.9715713 | -0.1145716 | -0.2071778 | 0.1404844 | 0.9833829 | 0.1149877 | 0.1905608 | -0.140824 | 0.9715221 |
| 21 | 176 | C | 1.3801 | -7.171 | 5.3461 | 0.7614275 | -0.2846163 | -0.5824274 | -0.1229605 | 0.8187386 | -0.5608457 | 0.6364816 | 0.4986589 | 0.5884135 |
| 22 | 188 | C | 6.8827 | 11.9212 | 9.2429 | 0.8660254 | -0.5 | 1.629566e-08 | 0.3950514 | 0.6842491 | 0.6129743 | -0.3064872 | -0.5308513 | 0.7901028 |
| 23 | 194 | C | -1.3793 | -16.6897 | -2.4311 | 0.7862335 | -0.1330104 | 0.6034444 | 0.07290877 | 0.9897055 | 0.1231561 | -0.6136133 | -0.05283304 | 0.7878372 |
| 24 | 206 | C | 0.0007 | -14.3159 | 1.4601 | 0.8715281 | -0.07836046 | 0.4840438 | 0.07982473 | 0.9966532 | 0.01761969 | -0.4838045 | 0.02328261 | 0.8748664 |
| 25 | 218 | C | 1.3798 | -11.9279 | 5.3516 | 0.8153296 | -0.2689766 | -0.5127272 | 0.02060642 | 0.898463 | -0.4385655 | 0.5786302 | 0.34701 | 0.7380861 |
| 26 | 230 | C | 2.7563 | -9.5377 | 9.2409 | 0.9649082 | 0.2262466 | 0.133284 | -0.07597813 | 0.7264199 | -0.6830384 | -0.2513553 | 0.6489426 | 0.7181183 |
| 27 | 242 | C | -6.8841 | -11.9237 | -6.3234 | 0.8660254 | -0.5 | 0.0 | 0.4644655 | 0.8044778 | 0.370253 | -0.1851265 | -0.3206485 | 0.928931 |
| 28 | 248 | C | 15.1461 | 2.3832 | -2.4281 | 0.9800014 | 0.1555372 | -0.1241182 | -0.0906989 | 0.9043208 | 0.4171063 | 0.1771182 | -0.3975073 | 0.9003427 |
| 29 | 260 | C | -5.498 | 4.7653 | -14.0987 | 0.6712678 | -0.097101 | 0.7348272 | -0.3950588 | 0.7919611 | 0.4655386 | -0.6271588 | -0.602801 | 0.4932574 |
| 30 | 272 | C | 2.7481 | 4.7599 | -14.0963 | 0.8660254 | -0.5 | 0.0 | 0.3552167 | 0.6152533 | -0.7037645 | 0.3518822 | 0.6094779 | 0.7104334 |
| 31 | 278 | C | -4.1244 | 2.3819 | -10.1929 | 0.7788455 | -0.4314746 | -0.4552245 | 0.4483011 | 0.8905522 | -0.07709025 | 0.4386637 | -0.1440363 | 0.8870331 |
| 32 | 290 | C | 1.3754 | 2.3823 | -6.2614 | 0.8660254 | -0.5 | 0.0 | 0.4386359 | 0.7597397 | 0.4799939 | -0.2399969 | -0.4156869 | 0.8772718 |
| 33 | 296 | C | 0.0 | 0.0 | 13.1119 | 1.0 | 0.0 | 0.0 | 0.0 | 1.0 | 0.0 | 0.0 | 0.0 | 1.0 |
| 34 | 298 | C | 1.3745 | 2.3807 | 17.016 | 0.8660254 | -0.5 | 0.0 | 0.4669866 | 0.8088446 | -0.3573429 | 0.1786714 | 0.309468 | 0.9339733 |
| 35 | 304 | C | -8.2578 | -14.303 | -10.2188 | 0.8660254 | -0.5 | 4.311743e-10 | 0.415183 | 0.719118 | 0.5572184 | -0.2786092 | -0.4825653 | 0.830366 |
| 36 | 310 | C | -5.5153 | -9.5528 | -2.431 | 0.8660254 | -0.5 | 0.0 | 0.4812549 | 0.8335579 | 0.2712472 | -0.1356236 | -0.234907 | 0.9625097 |
| 37 | 316 | C | -4.1391 | -7.1692 | 1.4576 | 0.8660254 | -0.5 | 0.0 | 0.4872219 | 0.8438931 | -0.2246315 | 0.1123157 | 0.1945366 | 0.9744438 |
| 38 | 322 | C | -2.7562 | -4.7739 | 5.3319 | 0.8660254 | -0.5 | 0.0 | 0.3554654 | 0.6156842 | 0.7032619 | -0.351631 | -0.6090427 | 0.7109309 |
| 39 | 328 | C | 9.633 | 16.6849 | 5.3473 | 0.8660254 | -0.5 | 0.0 | 0.4998201 | 0.8657139 | -0.02682009 | 0.01341004 | 0.02322688 | 0.9996403 |
| 40 | 334 | C | -6.8836 | -16.6851 | -6.3229 | 0.8823299 | -0.2037652 | -0.4242331 | 0.3099589 | 0.9299008 | 0.1980151 | 0.3541461 | -0.3062095 | 0.8836381 |
| 41 | 346 | C | -4.133 | -11.929 | 1.4624 | 0.9057291 | -0.2594673 | 0.335159 | 0.3577834 | 0.8919825 | -0.27633 | -0.2272574 | 0.3701944 | 0.9007276 |
| 42 | 358 | C | -2.753 | -9.5406 | 5.3495 | 0.6655075 | -0.6176389 | -0.4190728 | 0.3475927 | 0.7533286 | -0.5582789 | 0.6605143 | 0.2258721 | 0.7160326 |
| 43 | 370 | C | -1.3744 | -7.1494 | 9.2328 | 0.941394 | 0.00215273 | 0.3373022 | -0.2120122 | 0.7815377 | 0.5867279 | -0.2623513 | -0.6238543 | 0.7361913 |
| 44 | 382 | C | -2.7496 | -4.7625 | -17.9934 | 0.8660254 | -0.5 | 0.0 | 0.4218184 | 0.7306109 | -0.5369143 | 0.2684572 | 0.4649815 | 0.8436368 |
| 45 | 388 | C | 8.2567 | 4.762 | -10.2114 | 0.699669 | 0.1886233 | 0.6891187 | 0.4795452 | 0.5910025 | -0.6486543 | -0.5296222 | 0.7843069 | 0.3230527 |
| 46 | 400 | C | 9.6374 | 7.1501 | -6.3248 | 0.8424236 | -0.500094 | 0.2005704 | 0.5162864 | 0.642676 | -0.566053 | 0.1541779 | 0.5804082 | 0.7995971 |
| 47 | 412 | C | 11.0145 | 9.5383 | -2.4367 | 0.4863407 | -0.7002464 | -0.5226162 | 0.4921499 | 0.713747 | -0.4983509 | 0.7219842 | -0.01483712 | 0.6917504 |
| 48 | 424 | C | 4.1258 | 7.1461 | -10.2093 | 0.8660254 | -0.5 | 0.0 | 0.3794121 | 0.657161 | -0.6512956 | 0.3256478 | 0.5640385 | 0.7588241 |
| 49 | 430 | C | -6.8857 | 2.3868 | -6.3154 | 0.7266774 | -0.2847982 | 0.625164 | 0.2297297 | 0.9583703 | 0.16956 | -0.647429 | 0.02040331 | 0.7618526 |
| 50 | 442 | C | 2.7641 | 4.7876 | -2.4254 | 0.8660254 | -0.5 | -7.028319e-13 | 0.4626227 | 0.801286 | -0.3793692 | 0.1896846 | 0.3285433 | 0.9252454 |
| 51 | 448 | C | 0.0 | 0.0 | -21.8894 | 1.0 | 0.0 | 0.0 | 0.0 | 1.0 | 0.0 | 0.0 | 0.0 | 1.0 |
| 52 | 450 | C | 1.374 | 2.3799 | -17.992 | 0.8660254 | -0.5 | 0.0 | 0.4694676 | 0.8131417 | -0.3440943 | 0.1720471 | 0.2979944 | 0.9389351 |
| 53 | 456 | C | 5.5055 | 9.5357 | -6.3247 | 0.8660254 | -0.5 | 0.0 | 0.4070898 | 0.7051002 | -0.5806132 | 0.2903066 | 0.5028258 | 0.8141796 |
| 54 | 462 | C | 6.8845 | 11.9243 | -2.4383 | 0.8660254 | -0.5 | 0.0 | 0.4246685 | 0.7355475 | -0.5278509 | 0.2639254 | 0.4571323 | 0.8493371 |
| 55 | 468 | C | -1.3744 | -2.3805 | -14.092 | 0.8660254 | -0.5 | 0.0 | 0.4856041 | 0.8410909 | -0.2382324 | 0.1191162 | 0.2063153 | 0.9712082 |
| 56 | 474 | C | 6.894 | 7.1623 | -2.4324 | 0.7159206 | -0.2818544 | 0.6387611 | 0.5850176 | 0.7415183 | -0.328489 | -0.381067 | 0.6088585 | 0.695758 |
| 57 | 486 | C | 8.2666 | 9.5455 | 1.4572 | 0.6942536 | -0.5725552 | -0.4361107 | 0.6592023 | 0.7490659 | 0.06597401 | 0.2889019 | -0.3332879 | 0.8974714 |
| 58 | 498 | C | 4.1446 | 7.1787 | 1.4595 | 0.8660254 | -0.5 | 0.0 | 0.4931592 | 0.8541768 | 0.1648517 | -0.08242584 | -0.1427657 | 0.9863184 |
| 59 | 504 | C | -0.0 | 0.0 | -10.1821 | 1.0 | 0.0 | 0.0 | 0.0 | 1.0 | 0.0 | 0.0 | 0.0 | 1.0 |
| 60 | 506 | C | 5.5099 | 9.5434 | 5.3503 | 0.8660254 | -0.5 | 0.0 | 0.4516341 | 0.7822531 | 0.4290766 | -0.2145383 | -0.3715912 | 0.9032681 |

TABLE S9. Elements of rotation matrix from Cartesian to principal axes of hyperfine tensor with each lattice site for $^{13}C$ for the $GeV^0$ defect in diamond.

| Symmetry reduced # | Total # | Atom | x [Å] | y [Å] | z [Å] | $R_{xx}$ | $R_{xy}$ | $R_{xz}$ | $R_{yx}$ | $R_{yy}$ | $R_{yz}$ | $R_{zx}$ | $R_{zy}$ | $R_{zz}$ |
|---|---|---|---|---|---|---|---|---|---|---|---|---|---|---|
| 1 | 1 | GE | 0.0 | 0.0 | 0.0 | 1.0 | 0.0 | 0.0 | 0.0 | 1.0 | 0.0 | 0.0 | 0.0 | 1.0 |
| 2 | 2 | C | 1.3789 | 2.3883 | 5.2589 | 0.8660254 | -0.5 | 0.0 | 0.3722846 | 0.6448158 | -0.6675453 | 0.3337727 | 0.5781112 | 0.7445692 |
| 3 | 8 | C | 2.7532 | 4.7687 | 9.2216 | 0.8660254 | -0.5 | 3.240566e-13 | 0.4528059 | 0.7842828 | -0.4241077 | 0.2120539 | 0.3672881 | 0.9056117 |
| 4 | 14 | C | 4.1275 | 7.149 | 13.1276 | 0.8660254 | -0.5 | -1.443156e-09 | 0.4422441 | 0.7659893 | -0.4665625 | 0.2332813 | 0.404055 | 0.8844882 |
| 5 | 20 | C | -5.5041 | -9.5334 | -14.1065 | 0.8660254 | -0.5 | 0.0 | 0.4128296 | 0.7150419 | -0.5641691 | 0.2820846 | 0.4885848 | 0.8256593 |
| 6 | 26 | C | -4.1289 | -7.1515 | -10.2079 | 0.8660254 | -0.5 | 0.0 | 0.389915 | 0.6753526 | 0.6259913 | -0.3129956 | -0.5421244 | 0.77983 |
| 7 | 32 | C | -2.7569 | -4.775 | -6.3025 | 0.8660254 | -0.5 | 0.0 | 0.4497757 | 0.7790344 | 0.436815 | -0.2184075 | -0.3782928 | 0.8995514 |
| 8 | 38 | C | -1.496 | -2.5912 | -2.366 | 0.8660254 | -0.5 | 0.0 | 0.4727091 | 0.8187561 | 0.3258597 | -0.1629299 | -0.2822028 | 0.9454181 |
| 9 | 44 | C | -1.3732 | -2.3785 | 9.1964 | 0.8660254 | -0.5 | -8.734297e-14 | 0.4656466 | 0.8065235 | 0.3642707 | -0.1821354 | -0.3154677 | 0.9312931 |
| 10 | 50 | C | 4.1227 | 2.3812 | 13.1167 | 0.8078216 | -0.4677354 | -0.3586752 | 0.3618615 | 0.8738902 | -0.3246107 | 0.4652747 | 0.1324368 | 0.8752028 |
| 11 | 62 | C | -16.5178 | 4.7653 | 1.453 | 0.9475749 | -0.2274896 | 0.2243885 | 0.3142063 | 0.791068 | -0.5248674 | -0.05810469 | 0.5678555 | 0.8210749 |
| 12 | 74 | C | -4.1338 | -11.9187 | -10.2164 | 0.9741648 | -0.2251661 | 0.0174093 | 0.1603706 | 0.7439851 | 0.6486659 | -0.1590098 | -0.6291156 | 0.7608742 |
| 13 | 86 | C | -2.7568 | -9.5448 | -6.3246 | 0.9143319 | -0.2163363 | -0.3423387 | 0.3581083 | 0.8266503 | 0.4340596 | 0.1890916 | -0.5194689 | 0.8333045 |
| 14 | 98 | C | -1.3805 | -7.2233 | -2.4319 | 0.7097394 | -0.4746049 | 0.520596 | 0.375871 | 0.8801408 | 0.2899536 | -0.5958112 | -0.01011452 | 0.8030608 |
| 15 | 110 | C | 0.0229 | -4.8715 | 1.4549 | 0.8997404 | 0.05968194 | -0.4323255 | 0.03344114 | 0.9782649 | 0.2046447 | 0.4351424 | -0.1985845 | 0.8781886 |
| 16 | 122 | C | 8.2597 | 14.3062 | 1.4511 | 0.8660254 | -0.5 | 0.0 | 0.4763869 | 0.8251263 | -0.3036811 | 0.1518406 | 0.2629956 | 0.9527737 |
| 17 | 128 | C | -15.1427 | 2.3821 | 5.3485 | 0.9290502 | -0.2237403 | -0.2946286 | 0.3518816 | 0.7802918 | 0.5170338 | 0.114215 | -0.5840247 | 0.8036604 |
| 18 | 140 | C | -2.7578 | -14.3055 | -6.3243 | 0.8999538 | 0.1314946 | -0.4156831 | 0.06739544 | 0.9000152 | 0.4306163 | 0.4307448 | -0.4155499 | 0.80111 |
| 19 | 152 | C | -1.3784 | -11.9452 | -2.4326 | 0.6758316 | -0.3546317 | 0.6461332 | 0.2652082 | 0.9349286 | 0.2357397 | -0.6876891 | 0.01203951 | 0.7259055 |
| 20 | 164 | C | 0.0024 | -9.582 | 1.46 | 0.9744638 | -0.1159119 | -0.1923143 | 0.1383124 | 0.984545 | 0.1074282 | 0.1768899 | -0.1312843 | 0.9754355 |
| 21 | 176 | C | 1.3806 | -7.1707 | 5.3449 | 0.764412 | -0.2921573 | -0.5747333 | -0.1158199 | 0.8147072 | -0.5681884 | 0.6342397 | 0.5008956 | 0.5889343 |
| 22 | 188 | C | 6.8827 | 11.9212 | 9.2428 | 0.8660254 | -0.5 | 2.320696e-08 | 0.3923939 | 0.6796463 | 0.6197644 | -0.3098822 | -0.5367317 | 0.7847879 |
| 23 | 194 | C | -1.3792 | -16.6903 | -2.4309 | 0.7868241 | -0.1284165 | 0.6036697 | 0.06453986 | 0.9898712 | 0.1264504 | -0.6137935 | -0.06053347 | 0.7871424 |
| 24 | 206 | C | 0.0009 | -14.3173 | 1.4604 | 0.8681207 | -0.07397818 | 0.4908091 | 0.08061842 | 0.9967158 | 0.007637774 | -0.4897622 | 0.03293775 | 0.8712336 |
| 25 | 218 | C | 1.3799 | -11.9282 | 5.3516 | 0.815639 | -0.2793514 | -0.5066515 | 0.03088167 | 0.8954821 | -0.444025 | 0.5777364 | 0.3465179 | 0.739017 |
| 26 | 230 | C | 2.7565 | -9.5377 | 9.2406 | 0.9639238 | 0.2238836 | 0.1439686 | -0.06663011 | 0.7266037 | -0.6838183 | -0.2577038 | 0.6495561 | 0.7153081 |
| 27 | 242 | C | -6.884 | -11.9234 | -6.323 | 0.8660254 | -0.5 | 0.0 | 0.4634955 | 0.8027977 | 0.3750836 | -0.1875418 | -0.3248319 | 0.926991 |
| 28 | 248 | C | 15.1461 | 2.3832 | -2.4276 | 0.9806872 | 0.1577367 | -0.1156361 | -0.09660336 | 0.9047408 | 0.4148636 | 0.1700599 | -0.3956806 | 0.9025057 |
| 29 | 260 | C | -5.4977 | 4.7651 | -14.098 | 0.6694334 | -0.1017639 | 0.7358689 | -0.393385 | 0.7917229 | 0.4673576 | -0.6301644 | -0.6023446 | 0.4899734 |
| 30 | 272 | C | 2.7481 | 4.7598 | -14.0954 | 0.8660254 | -0.5 | 0.0 | 0.3540445 | 0.613223 | -0.7061232 | 0.3530616 | 0.6115206 | 0.708089 |
| 31 | 278 | C | -4.1236 | 2.3815 | -10.191 | 0.7666208 | -0.4539221 | -0.4541446 | 0.4681176 | 0.8792156 | -0.08857682 | 0.439498 | -0.1446882 | 0.8865139 |
| 32 | 290 | C | 1.3734 | 2.3788 | -6.2549 | 0.8660254 | -0.5 | 0.0 | 0.4388508 | 0.7601118 | 0.4792077 | -0.2396038 | -0.415006 | 0.8777016 |
| 33 | 296 | C | 0.0 | 0.0 | 13.1092 | 1.0 | 0.0 | 0.0 | 0.0 | 1.0 | 0.0 | 0.0 | 0.0 | 1.0 |
| 34 | 298 | C | 1.3745 | 2.3806 | 17.015 | 0.8660254 | -0.5 | 0.0 | 0.4690024 | 0.812336 | -0.3466222 | 0.1733111 | 0.3001836 | 0.9380048 |
| 35 | 304 | C | -8.2579 | -14.303 | -10.219 | 0.8660254 | -0.5 | 5.516068e-10 | 0.4087688 | 0.7080083 | 0.5758753 | -0.2879376 | -0.4987226 | 0.8175376 |
| 36 | 310 | C | -5.5149 | -9.5521 | -2.4301 | 0.8660254 | -0.5 | 0.0 | 0.4817069 | 0.8343408 | 0.2680185 | -0.1340092 | -0.2321108 | 0.9634138 |
| 37 | 316 | C | -4.1373 | -7.1659 | 1.4576 | 0.8660254 | -0.5 | 0.0 | 0.486298 | 0.8422928 | -0.232502 | 0.116251 | 0.2013526 | 0.9725959 |
| 38 | 322 | C | -2.7548 | -4.7715 | 5.3286 | 0.8660254 | -0.5 | 0.0 | 0.355569 | 0.6158636 | 0.7030524 | -0.3515262 | -0.6088612 | 0.711138 |
| 39 | 328 | C | 9.6331 | 16.6849 | 5.347 | 0.8660254 | -0.5 | 0.0 | 0.499752 | 0.8655959 | -0.031491 | 0.0157455 | 0.027272 | 0.999504 |
| 40 | 334 | C | -6.8836 | -16.685 | -6.3228 | 0.873901 | -0.1799192 | -0.4515817 | 0.298761 | 0.9316098 | 0.2069904 | 0.3834564 | -0.3158042 | 0.8678876 |
| 41 | 346 | C | -4.1328 | -11.9285 | 1.4628 | 0.9049686 | -0.2578616 | 0.3384364 | 0.3593638 | 0.8890882 | -0.2835133 | -0.2277926 | 0.3781924 | 0.8972631 |
| 42 | 358 | C | -2.7527 | -9.5397 | 5.3491 | 0.6654177 | -0.6148734 | -0.4232611 | 0.3463128 | 0.7565885 | -0.5546542 | 0.6612766 | 0.222496 | 0.7163859 |
| 43 | 370 | C | -1.3744 | -7.1489 | 9.2313 | 0.9354548 | 0.02439739 | 0.3526032 | -0.2382993 | 0.7803075 | 0.5782159 | -0.261032 | -0.62492 | 0.7357563 |
| 44 | 382 | C | -2.7495 | -4.7624 | -17.9928 | 0.8660254 | -0.5 | 0.0 | 0.4239666 | 0.7343317 | -0.530103 | 0.2650515 | 0.4590827 | 0.8479332 |
| 45 | 388 | C | 8.2563 | 4.762 | -10.211 | 0.7047201 | 0.1797714 | 0.6863322 | 0.4785532 | 0.5937328 | -0.6468912 | -0.5237905 | 0.7843236 | 0.3323853 |
| 46 | 400 | C | 9.637 | 7.1501 | -6.3247 | 0.8448351 | -0.4936353 | 0.206344 | 0.5148807 | 0.6452887 | -0.5643584 | 0.1454358 | 0.5830323 | 0.7993258 |
| 47 | 412 | C | 11.0145 | 9.5385 | -2.437 | 0.485306 | -0.7007654 | -0.5228824 | 0.4922871 | 0.7132286 | -0.4989573 | 0.7225867 | -0.01526125 | 0.6911118 |
| 48 | 424 | C | 4.1257 | 7.1459 | -10.2087 | 0.8660254 | -0.5 | 0.0 | 0.3802702 | 0.6586472 | -0.6492907 | 0.3246454 | 0.5623023 | 0.7605403 |
| 49 | 430 | C | -6.8841 | 2.3862 | -6.314 | 0.7298636 | -0.2754263 | 0.6256512 | 0.2243016 | 0.9610583 | 0.1614176 | -0.645746 | 0.02252176 | 0.7632201 |
| 50 | 442 | C | 2.7612 | 4.7826 | -2.4236 | 0.8660254 | -0.5 | -2.430259e-13 | 0.462656 | 0.8013437 | -0.3792066 | 0.1896033 | 0.3284025 | 0.925312 |
| 51 | 448 | C | 0.0 | 0.0 | -21.8893 | 1.0 | 0.0 | 0.0 | 0.0 | 1.0 | 0.0 | 0.0 | 0.0 | 1.0 |
| 52 | 450 | C | 1.374 | 2.3798 | -17.9913 | 0.8660254 | -0.5 | 0.0 | 0.4551944 | 0.7884198 | -0.413754 | 0.206877 | 0.3583214 | 0.9103887 |
| 53 | 456 | C | 5.5053 | 9.5355 | -6.3246 | 0.8660254 | -0.5 | 0.0 | 0.4080126 | 0.7066985 | -0.5780164 | 0.2890082 | 0.5005769 | 0.8160251 |
| 54 | 462 | C | 6.8845 | 11.9243 | -2.4388 | 0.8660254 | -0.5 | 0.0 | 0.4251281 | 0.7363435 | -0.5263691 | 0.2631845 | 0.455849 | 0.8502562 |
| 55 | 468 | C | -1.3743 | -2.3803 | -14.0905 | 0.8660254 | -0.5 | 0.0 | 0.4855185 | 0.8409427 | -0.2389293 | 0.1194646 | 0.2069188 | 0.971037 |
| 56 | 474 | C | 6.8934 | 7.1616 | -2.432 | 0.7089925 | -0.2743809 | 0.6496497 | 0.5869746 | 0.7402019 | -0.3279665 | -0.3908841 | 0.6138537 | 0.6858522 |
| 57 | 486 | C | 8.2668 | 9.5458 | 1.4571 | 0.692804 | -0.5742547 | -0.4361814 | 0.6586026 | 0.750223 | 0.05837803 | 0.2937095 | -0.3277147 | 0.8979631 |
| 58 | 498 | C | 4.1448 | 7.1789 | 1.4591 | 0.8660254 | -0.5 | 0.0 | 0.4938466 | 0.8553675 | 0.1564034 | -0.07820168 | -0.1354493 | 0.9876933 |
| 59 | 504 | C | -0.0 | 0.0 | -10.1787 | 1.0 | 0.0 | 0.0 | 0.0 | 1.0 | 0.0 | 0.0 | 0.0 | 1.0 |
| 60 | 506 | C | 5.5098 | 9.5432 | 5.3499 | 0.8660254 | -0.5 | 0.0 | 0.4511617 | 0.781435 | 0.4310597 | -0.2155298 | -0.3733086 | 0.9023234 |

TABLE S10. Elements of rotation matrix from Cartesian to principal axes of hyperfine tensor with each lattice site for $^{13}C$ for the $GeV^{-}$ defect in diamond.

| Symmetry reduced # | Total # | Atom | x [Å] | y [Å] | z [Å] | $R_{xx}$ | $R_{xy}$ | $R_{xz}$ | $R_{yx}$ | $R_{yy}$ | $R_{yz}$ | $R_{zx}$ | $R_{zy}$ | $R_{zz}$ |
|---|---|---|---|---|---|---|---|---|---|---|---|---|---|---|
| 1 | 1 | SN117 | 0.0 | 0.0 | 0.0 | 1.0 | 0.0 | 0.0 | 0.0 | 1.0 | 0.0 | 0.0 | 0.0 | 1.0 |
| 1 | 1 | SN119 | 0.0 | 0.0 | 0.0 | 1.0 | 0.0 | 0.0 | 0.0 | 1.0 | 0.0 | 0.0 | 0.0 | 1.0 |
| 2 | 2 | C | 1.3908 | 2.4089 | 5.3093 | 0.8660254 | -0.5 | 0.0 | 0.3704379 | 0.6416173 | -0.6716421 | 0.335821 | 0.5816591 | 0.7408758 |
| 3 | 8 | C | 2.7577 | 4.7765 | 9.2392 | 0.8660254 | -0.5 | 3.057041e-13 | 0.4624302 | 0.8009527 | -0.3803066 | 0.1901533 | 0.3293551 | 0.9248605 |
| 4 | 14 | C | 4.1287 | 7.1512 | 13.1323 | 0.8660254 | -0.5 | -4.169516e-10 | 0.4464253 | 0.7732313 | -0.450353 | 0.2251765 | 0.3900171 | 0.8928506 |
| 5 | 20 | C | -5.5046 | -9.5343 | -14.1078 | 0.8660254 | -0.5 | 0.0 | 0.4119221 | 0.71347 | -0.5668163 | 0.2834082 | 0.4908773 | 0.8238442 |
| 6 | 26 | C | -4.132 | -7.1569 | -10.2164 | 0.8660254 | -0.5 | 0.0 | 0.3934731 | 0.6815153 | 0.6170217 | -0.3085109 | -0.5343565 | 0.7869461 |
| 7 | 32 | C | -2.7671 | -4.7927 | -6.3317 | 0.8660254 | -0.5 | 0.0 | 0.4479357 | 0.7758474 | 0.4443133 | -0.2221567 | -0.3847866 | 0.8958715 |
| 8 | 38 | C | -1.5554 | -2.694 | -2.4667 | 0.8660254 | -0.5 | 0.0 | 0.4725138 | 0.8184178 | 0.3269908 | -0.1634954 | -0.2831823 | 0.9450275 |
| 9 | 44 | C | -1.3749 | -2.3814 | 9.2111 | 0.8660254 | -0.5 | 2.387604e-14 | 0.465679 | 0.8065797 | 0.3641047 | -0.1820523 | -0.3153239 | 0.931358 |
| 10 | 50 | C | 4.1234 | 2.3818 | 13.1228 | 0.8063455 | -0.474459 | -0.3531227 | 0.3720348 | 0.8710256 | -0.3207874 | 0.4597794 | 0.1272915 | 0.8788628 |
| 11 | 62 | C | -16.5187 | 4.7653 | 1.4547 | 0.9418535 | -0.2067107 | 0.26492 | 0.3198624 | 0.7930921 | -0.518356 | -0.1029562 | 0.5729534 | 0.8130956 |
| 12 | 74 | C | -4.1356 | -11.9205 | -10.2174 | 0.9786764 | -0.1961774 | 0.06088433 | 0.1095404 | 0.7491984 | 0.6532249 | -0.1737624 | -0.6326265 | 0.7547121 |
| 13 | 86 | C | -2.759 | -9.5511 | -6.3289 | 0.934507 | -0.2219934 | -0.2782367 | 0.3304882 | 0.8314456 | 0.446627 | 0.1321904 | -0.50933 | 0.8503579 |
| 14 | 98 | C | -1.3844 | -7.2453 | -2.4378 | 0.6733409 | -0.4597553 | 0.5789967 | 0.3634077 | 0.8878137 | 0.2823501 | -0.6438532 | 0.02029402 | 0.7648799 |
| 15 | 110 | C | 0.0194 | -4.9003 | 1.4642 | 0.8930603 | 0.109884 | -0.4363127 | 0.004840524 | 0.9673171 | 0.2535235 | 0.4499109 | -0.2285238 | 0.8633406 |
| 16 | 122 | C | 8.2603 | 14.3072 | 1.4537 | 0.8660254 | -0.5 | 0.0 | 0.4718157 | 0.8172087 | -0.3309982 | 0.1654991 | 0.2866529 | 0.9436314 |
| 17 | 128 | C | -15.1445 | 2.3817 | 5.3492 | 0.9241428 | -0.2389702 | -0.2980826 | 0.3675129 | 0.769218 | 0.5227217 | 0.1043756 | -0.5926187 | 0.7986919 |
| 18 | 140 | C | -2.7598 | -14.3075 | -6.3246 | 0.8999211 | 0.1824088 | -0.396067 | 0.01602057 | 0.8938564 | 0.448067 | 0.4357584 | -0.4095702 | 0.801478 |
| 19 | 152 | C | -1.38 | -11.9523 | -2.4342 | 0.6953518 | -0.3512668 | 0.6269749 | 0.2609915 | 0.9362754 | 0.2350996 | -0.6696038 | 0.0001581587 | 0.7427184 |
| 20 | 164 | C | 0.0013 | -9.5945 | 1.4604 | 0.9652888 | -0.1344573 | -0.2239168 | 0.1665438 | 0.9772767 | 0.131124 | 0.2011981 | -0.1638644 | 0.9657473 |
| 21 | 176 | C | 1.3818 | -7.1792 | 5.3538 | 0.7493942 | -0.3327629 | -0.5724309 | -0.07247724 | 0.8181165 | -0.5704668 | 0.6581454 | 0.4689927 | 0.5889741 |
| 22 | 188 | C | 6.8836 | 11.9227 | 9.2433 | 0.8660254 | -0.5 | 3.569936e-08 | 0.3910048 | 0.6772403 | 0.6232663 | -0.3116331 | -0.5397644 | 0.7820097 |
| 23 | 194 | C | -1.3804 | -16.6918 | -2.4309 | 0.7856932 | -0.1286056 | 0.6051007 | 0.05428365 | 0.9887116 | 0.139652 | -0.6162301 | -0.07687655 | 0.7838051 |
| 24 | 206 | C | 0.0012 | -14.3209 | 1.4601 | 0.8691685 | -0.08531928 | 0.4871004 | 0.08890573 | 0.9959147 | 0.01580099 | -0.4864585 | 0.0295723 | 0.8732031 |
| 25 | 218 | C | 1.3812 | -11.9319 | 5.3529 | 0.5875321 | 0.3378819 | 0.7352836 | 0.04633845 | 0.8931145 | -0.4474362 | -0.807873 | 0.296955 | 0.5090765 |
| 26 | 230 | C | 2.7582 | -9.5405 | 9.2443 | 0.9664362 | 0.2026392 | 0.1579191 | -0.04515904 | 0.7391187 | -0.6720596 | -0.2529066 | 0.6423713 | 0.7234621 |
| 27 | 242 | C | -6.8854 | -11.9258 | -6.3242 | 0.8660254 | -0.5 | 0.0 | 0.4630903 | 0.802096 | 0.3770801 | -0.1885401 | -0.326561 | 0.9261806 |
| 28 | 248 | C | 15.1485 | 2.3833 | -2.4293 | 0.9826727 | 0.1609678 | -0.09188988 | -0.1088485 | 0.9024453 | 0.4168267 | 0.1500213 | -0.3996021 | 0.9043295 |
| 29 | 260 | C | -5.4976 | 4.7662 | -14.1013 | 0.6610805 | -0.1063251 | 0.7427433 | -0.3976164 | 0.7898379 | 0.4669661 | -0.636297 | -0.6040291 | 0.4798698 |
| 30 | 272 | C | 2.7478 | 4.7594 | -14.0995 | 0.8660254 | -0.5 | 0.0 | 0.354819 | 0.6145645 | 0.7045665 | -0.3522832 | -0.6101725 | 0.709638 |
| 31 | 278 | C | -4.1265 | 2.3838 | -10.2003 | 0.7952919 | -0.3967319 | -0.4583826 | 0.4146795 | 0.9075682 | -0.06603645 | 0.4422123 | -0.1375636 | 0.8862982 |
| 32 | 290 | C | 1.3783 | 2.3873 | -6.2759 | 0.8660254 | -0.5 | 0.0 | 0.4327572 | 0.7495575 | 0.5008839 | -0.2504419 | -0.4337782 | 0.8655145 |
| 33 | 296 | C | 0.0 | 0.0 | 13.1158 | 1.0 | 0.0 | 0.0 | 0.0 | 1.0 | 0.0 | 0.0 | 0.0 | 1.0 |
| 34 | 298 | C | 1.3744 | 2.3804 | 17.0179 | 0.8660254 | -0.5 | 0.0 | 0.4704454 | 0.8148354 | -0.3387098 | 0.1693549 | 0.2933313 | 0.9408909 |
| 35 | 304 | C | -8.2584 | -14.3039 | -10.2185 | 0.8660254 | -0.5 | 7.744339e-10 | 0.4015309 | 0.695472 | 0.5958956 | -0.2979478 | -0.5160608 | 0.8030619 |
| 36 | 310 | C | -5.5184 | -9.5581 | -2.432 | 0.8660254 | -0.5 | 0.0 | 0.484146 | 0.8385655 | 0.2498209 | -0.1249105 | -0.2163513 | 0.9682921 |
| 37 | 316 | C | -4.142 | -7.1742 | 1.4585 | 0.8660254 | -0.5 | 0.0 | 0.475528 | 0.8236387 | -0.3090184 | 0.1545092 | 0.2676178 | 0.9510561 |
| 38 | 322 | C | -2.7579 | -4.7769 | 5.3383 | 0.8660254 | -0.5 | 0.0 | 0.3591487 | 0.6220638 | -0.6957362 | 0.3478681 | 0.6025252 | 0.7182974 |
| 39 | 328 | C | 9.6333 | 16.6854 | 5.3479 | 0.8660254 | -0.5 | 0.0 | 0.4996929 | 0.8654934 | -0.03504472 | 0.01752236 | 0.03034962 | 0.9993857 |
| 40 | 334 | C | -6.8845 | -16.6857 | -6.3233 | 0.8645515 | -0.1465212 | -0.4807101 | 0.2793787 | 0.9352471 | 0.2173946 | 0.4177298 | -0.322249 | 0.8495042 |
| 41 | 346 | C | -4.134 | -11.9319 | 1.4616 | 0.8995434 | -0.2474207 | 0.3600066 | 0.3617929 | 0.8838234 | -0.296584 | -0.2448012 | 0.397038 | 0.8845526 |
| 42 | 358 | C | -2.753 | -9.5427 | 5.3505 | 0.6449764 | -0.6235376 | -0.4418216 | 0.3558348 | 0.7566894 | -0.5484549 | 0.676304 | 0.196525 | 0.7099231 |
| 43 | 370 | C | -1.3741 | -7.1508 | 9.2363 | 0.9322073 | 0.01430974 | 0.3616417 | -0.237661 | 0.777801 | 0.5818443 | -0.2729592 | -0.6283476 | 0.7284727 |
| 44 | 382 | C | -2.7493 | -4.7619 | -17.9944 | 0.8660254 | -0.5 | 0.0 | 0.4258086 | 0.7375221 | -0.5241642 | 0.2620821 | 0.4539395 | 0.8516172 |
| 45 | 388 | C | 8.2582 | 4.7614 | -10.2133 | 0.7089295 | 0.1640393 | 0.6859373 | 0.4831073 | 0.5956284 | -0.641743 | -0.5138348 | 0.786332 | 0.34301 |
| 46 | 400 | C | 9.6393 | 7.15 | -6.3249 | 0.844805 | -0.4923493 | 0.2095152 | 0.5165 | 0.6480906 | -0.5596483 | 0.1397576 | 0.5810084 | 0.8018086 |
| 47 | 412 | C | 11.0164 | 9.539 | -2.4354 | 0.4854666 | -0.6995583 | -0.5243476 | 0.4860986 | 0.7144969 | -0.5031921 | 0.7266569 | -0.01060166 | 0.6869187 |
| 48 | 424 | C | 4.1258 | 7.1461 | -10.2115 | 0.8660254 | -0.5 | 0.0 | 0.3824318 | 0.6623914 | -0.6441922 | 0.3220961 | 0.5578868 | 0.7648637 |
| 49 | 430 | C | -6.8887 | 2.3885 | -6.3195 | 0.7416614 | -0.2659521 | 0.6157985 | 0.2239907 | 0.9635384 | 0.1463624 | -0.6322709 | 0.0293818 | 0.7741901 |
| 50 | 442 | C | 2.7685 | 4.7952 | -2.4323 | 0.8660254 | -0.5 | -1.017434e-12 | 0.4639458 | 0.8035776 | -0.3728503 | 0.1864252 | 0.3228979 | 0.9278915 |
| 51 | 448 | C | 0.0 | 0.0 | -21.8899 | 1.0 | 0.0 | 0.0 | 0.0 | 1.0 | 0.0 | 0.0 | 0.0 | 1.0 |
| 52 | 450 | C | 1.3737 | 2.3793 | -17.9935 | 0.8660254 | -0.5 | 0.0 | 0.4295901 | 0.7440719 | -0.5116731 | 0.2558366 | 0.4431219 | 0.8591802 |
| 53 | 456 | C | 5.5059 | 9.5365 | -6.3246 | 0.8660254 | -0.5 | 0.0 | 0.4106519 | 0.7112699 | -0.5704911 | 0.2852456 | 0.4940598 | 0.8213038 |
| 54 | 462 | C | 6.8853 | 11.9257 | -2.4366 | 0.8660254 | -0.5 | 0.0 | 0.4248608 | 0.7358804 | -0.5272317 | 0.2636159 | 0.4565961 | 0.8497215 |
| 55 | 468 | C | -1.3745 | -2.3806 | -14.095 | 0.8660254 | -0.5 | 0.0 | 0.4859454 | 0.8416822 | -0.2354319 | 0.117716 | 0.20389 | 0.9718908 |
| 56 | 474 | C | 6.8981 | 7.1656 | -2.433 | 0.4586538 | -0.637166 | -0.6193999 | 0.5822297 | 0.742055 | -0.3322092 | 0.6713012 | -0.208264 | 0.7113233 |
| 57 | 486 | C | 8.2695 | 9.5487 | 1.4581 | 0.6927124 | -0.5774334 | -0.4321114 | 0.6543833 | 0.7551053 | 0.03998141 | 0.303203 | -0.3104621 | 0.9009335 |
| 58 | 498 | C | 4.1493 | 7.1867 | 1.4601 | 0.8660254 | -0.5 | 0.0 | 0.4977814 | 0.8621826 | 0.09410034 | -0.04705017 | -0.08149329 | 0.9955627 |
| 59 | 504 | C | 0.0 | 0.0 | -10.188 | 1.0 | 0.0 | 0.0 | 0.0 | 1.0 | 0.0 | 0.0 | 0.0 | 1.0 |
| 60 | 506 | C | 5.5115 | 9.5463 | 5.352 | 0.8660254 | -0.5 | 0.0 | 0.4533117 | 0.7851589 | 0.4219406 | -0.2109703 | -0.3654113 | 0.9066235 |

TABLE S11. Elements of rotation matrix from Cartesian to principal axes of hyperfine tensor with each lattice site for $^{13}C$ for the $SnV^0$ defect in diamond.

| Symmetry reduced # | Total # | Atom | x [Å] | y [Å] | z [Å] | $R_{xx}$ | $R_{xy}$ | $R_{xz}$ | $R_{yx}$ | $R_{yy}$ | $R_{yz}$ | $R_{zx}$ | $R_{zy}$ | $R_{zz}$ |
|---|---|---|---|---|---|---|---|---|---|---|---|---|---|---|
| 1 | 1 | SN117 | 0.0 | 0.0 | 0.0 | 1.0 | 0.0 | 0.0 | 0.0 | 1.0 | 0.0 | 0.0 | 0.0 | 1.0 |
| 1 | 1 | SN119 | 0.0 | 0.0 | 0.0 | 1.0 | 0.0 | 0.0 | 0.0 | 1.0 | 0.0 | 0.0 | 0.0 | 1.0 |
| 2 | 2 | C | 1.3934 | 2.4134 | 5.3018 | 0.8660254 | -0.5 | 0.0 | 0.3854318 | 0.6675874 | -0.6370004 | 0.3185002 | 0.5516585 | 0.7708635 |
| 3 | 8 | C | 2.7589 | 4.7785 | 9.2385 | 0.8660254 | -0.5 | 3.202915e-13 | 0.462824 | 0.8016346 | -0.3783859 | 0.189193 | 0.3276918 | 0.9256479 |
| 4 | 14 | C | 4.129 | 7.1517 | 13.1322 | 0.8660254 | -0.5 | -6.152817e-10 | 0.4451428 | 0.77101 | -0.4554025 | 0.2277013 | 0.3943902 | 0.8902856 |
| 5 | 20 | C | -5.5047 | -9.5344 | -14.1079 | 0.8660254 | -0.5 | 0.0 | 0.4113609 | 0.712498 | -0.5684441 | 0.2842221 | 0.492287 | 0.8227219 |
| 6 | 26 | C | -4.1321 | -7.1569 | -10.2171 | 0.8660254 | -0.5 | 0.0 | 0.3909054 | 0.6770681 | 0.6235157 | -0.3117578 | -0.5399804 | 0.7818109 |
| 7 | 32 | C | -2.7654 | -4.7899 | -6.3322 | 0.8660254 | -0.5 | 0.0 | 0.4470794 | 0.7743643 | 0.4477498 | -0.2238749 | -0.3877627 | 0.8941589 |
| 8 | 38 | C | -1.555 | -2.6933 | -2.4597 | 0.8660254 | -0.5 | 0.0 | 0.4720707 | 0.8176504 | 0.3295406 | -0.1647703 | -0.2853905 | 0.9441414 |
| 9 | 44 | C | -1.3747 | -2.3811 | 9.2068 | 0.8660254 | -0.5 | 9.096951e-14 | 0.4659126 | 0.8069843 | 0.3629075 | -0.1814537 | -0.3142871 | 0.9318252 |
| 10 | 50 | C | 4.1232 | 2.3817 | 13.1214 | 0.8063741 | -0.4727783 | -0.3553047 | 0.3703817 | 0.872083 | -0.3198259 | 0.4610619 | 0.126301 | 0.8783336 |
| 11 | 62 | C | -16.5191 | 4.7653 | 1.4544 | 0.9384455 | -0.1933998 | 0.2862107 | 0.321289 | 0.793002 | -0.517611 | -0.1268598 | 0.5777061 | 0.8063264 |
| 12 | 74 | C | -4.1358 | -11.9204 | -10.2173 | 0.9800503 | -0.1808732 | 0.08237894 | 0.08327552 | 0.7500519 | 0.6561153 | -0.1804622 | -0.6361659 | 0.7501509 |
| 13 | 86 | C | -2.7586 | -9.5504 | -6.3282 | 0.938953 | -0.2154663 | -0.2682191 | 0.3203501 | 0.831858 | 0.4531977 | 0.1254714 | -0.5114553 | 0.8501002 |
| 14 | 98 | C | -1.3811 | -7.2479 | -2.4342 | 0.6716806 | -0.4593636 | 0.5812317 | 0.3612827 | 0.8880451 | 0.2843427 | -0.6467766 | 0.01900153 | 0.7624428 |
| 15 | 110 | C | 0.028 | -4.9033 | 1.4676 | 0.8983325 | 0.09553405 | -0.4288029 | 0.02327142 | 0.9643505 | 0.2636031 | 0.4386993 | -0.2467821 | 0.8640842 |
| 16 | 122 | C | 8.2605 | 14.3075 | 1.4531 | 0.8660254 | -0.5 | 0.0 | 0.4702176 | 0.8144408 | -0.3399729 | 0.1699865 | 0.2944252 | 0.9404352 |
| 17 | 128 | C | -15.1447 | 2.3817 | 5.349 | 0.9203711 | -0.2439501 | -0.305623 | 0.3780391 | 0.754963 | 0.5358333 | 0.1000174 | -0.6087029 | 0.7870688 |
| 18 | 140 | C | -2.76 | -14.3076 | -6.3246 | 0.8964856 | 0.2111071 | -0.3895476 | -0.01060451 | 0.8891667 | 0.4574605 | 0.4429459 | -0.4059758 | 0.7993638 |
| 19 | 152 | C | -1.3793 | -11.9546 | -2.4337 | 0.7002882 | -0.3471798 | 0.6237489 | 0.2553495 | 0.9377825 | 0.2352884 | -0.6666282 | -0.005495732 | 0.7453702 |
| 20 | 164 | C | 0.0028 | -9.5985 | 1.4611 | 0.9672092 | -0.1369623 | -0.2138873 | 0.1660321 | 0.9782436 | 0.1243895 | 0.1921972 | -0.1558228 | 0.9689063 |
| 21 | 176 | C | 1.3823 | -7.1797 | 5.3525 | 0.7535668 | -0.338586 | -0.5634683 | -0.06548198 | 0.8142281 | -0.5768403 | 0.6541018 | 0.4715848 | 0.591404 |
| 22 | 188 | C | 6.8837 | 11.9229 | 9.2431 | 0.8660254 | -0.4999999 | 4.65565e-08 | 0.3893714 | 0.6744113 | 0.6273431 | -0.3136715 | -0.5432951 | 0.778743 |
| 23 | 194 | C | -1.3804 | -16.6926 | -2.4308 | 0.7861183 | -0.1241382 | 0.6054815 | 0.04503049 | 0.9885226 | 0.1442061 | -0.6164336 | -0.08609793 | 0.7826856 |
| 24 | 206 | C | 0.0016 | -14.3227 | 1.4604 | 0.8672479 | -0.08040892 | 0.4913405 | 0.08911143 | 0.9960053 | 0.005710924 | -0.489837 | 0.03883127 | 0.8709488 |
| 25 | 218 | C | 1.3815 | -11.9326 | 5.3529 | 0.5830532 | 0.338417 | 0.7385952 | 0.05425889 | 0.8908642 | -0.4510176 | -0.8106201 | 0.3030426 | 0.5010591 |
| 26 | 230 | C | 2.7585 | -9.5408 | 9.244 | 0.9653955 | 0.2010076 | 0.1661548 | -0.03811539 | 0.7390311 | -0.6725922 | -0.2579897 | 0.6429844 | 0.7211188 |
| 27 | 242 | C | -6.8852 | -11.9256 | -6.3238 | 0.8660254 | -0.5 | 0.0 | 0.4621486 | 0.8004649 | 0.3816733 | -0.1908367 | -0.3305388 | 0.9242973 |
| 28 | 248 | C | 15.1487 | 2.3833 | -2.4288 | 0.9831664 | 0.1634323 | -0.08169306 | -0.1149311 | 0.9007569 | 0.418841 | 0.1420378 | -0.4024013 | 0.9043774 |
| 29 | 260 | C | -5.4973 | 4.7661 | -14.1008 | 0.66054 | -0.109467 | 0.7427677 | -0.3970312 | 0.7887364 | 0.4693199 | -0.6372229 | -0.6049065 | 0.4775302 |
| 30 | 272 | C | 2.7477 | 4.7592 | -14.0988 | 0.8660254 | -0.5 | 0.0 | 0.356154 | 0.6168768 | 0.701867 | -0.3509335 | -0.6078346 | 0.712308 |
| 31 | 278 | C | -4.1259 | 2.3838 | -10.1988 | 0.784551 | -0.4188152 | -0.4572456 | 0.4347737 | 0.8973337 | -0.07592168 | 0.442099 | -0.1392339 | 0.8860939 |
| 32 | 290 | C | 1.3767 | 2.3845 | -6.2706 | 0.8660254 | -0.5 | 0.0 | 0.4330668 | 0.7500937 | 0.4998125 | -0.2499063 | -0.4328503 | 0.8661336 |
| 33 | 296 | C | 0.0 | 0.0 | 13.1136 | 1.0 | 0.0 | 0.0 | 0.0 | 1.0 | 0.0 | 0.0 | 0.0 | 1.0 |
| 34 | 298 | C | 1.3743 | 2.3803 | 17.017 | 0.8660254 | -0.5 | 0.0 | 0.4717947 | 0.8171724 | -0.3311179 | 0.165559 | 0.2867565 | 0.9435894 |
| 35 | 304 | C | -8.2584 | -14.304 | -10.2186 | 0.8660254 | -0.5 | 7.702008e-10 | 0.3970543 | 0.6877182 | 0.607776 | -0.303888 | -0.5263494 | 0.7941085 |
| 36 | 310 | C | -5.5181 | -9.5576 | -2.431 | 0.8660254 | -0.5 | 0.0 | 0.4847957 | 0.8396909 | 0.2447291 | -0.1223646 | -0.2119416 | 0.9695915 |
| 37 | 316 | C | -4.1408 | -7.1721 | 1.4588 | 0.8660254 | -0.5 | 0.0 | 0.4747001 | 0.8222047 | -0.3140688 | 0.1570344 | 0.2719915 | 0.9494002 |
| 38 | 322 | C | -2.7569 | -4.7751 | 5.3354 | 0.8660254 | -0.5 | 0.0 | 0.3592754 | 0.6222833 | -0.6954744 | 0.3477372 | 0.6022985 | 0.7185509 |
| 39 | 328 | C | 9.6334 | 16.6855 | 5.3477 | 0.8660254 | -0.5 | 0.0 | 0.4994855 | 0.8651343 | -0.04535275 | 0.02267638 | 0.03927663 | 0.998971 |
| 40 | 334 | C | -6.8846 | -16.6857 | -6.3231 | 0.8596004 | -0.1269046 | -0.494957 | 0.2667701 | 0.9376295 | 0.2229006 | 0.4357991 | -0.3236452 | 0.839841 |
| 41 | 346 | C | -4.1339 | -11.9319 | 1.462 | 0.8982504 | -0.2441545 | 0.3654241 | 0.3622747 | 0.8820778 | -0.3011573 | -0.2488036 | 0.4028986 | 0.8807778 |
| 42 | 358 | C | -2.7528 | -9.5424 | 5.3502 | 0.6454523 | -0.6206806 | -0.445137 | 0.3547496 | 0.7597289 | -0.5449447 | 0.6764201 | 0.1938237 | 0.7105549 |
| 43 | 370 | C | -1.3739 | -7.1505 | 9.2349 | 0.9269199 | 0.03276871 | 0.3738257 | -0.2590266 | 0.7766675 | 0.5741888 | -0.2715229 | -0.6290578 | 0.7283966 |
| 44 | 382 | C | -2.7492 | -4.7617 | -17.9939 | 0.8660254 | -0.5 | 0.0 | 0.427283 | 0.7400758 | -0.5193429 | 0.2596714 | 0.4497641 | 0.854566 |
| 45 | 388 | C | 8.258 | 4.7611 | -10.2128 | 0.7143326 | 0.155496 | 0.6823122 | 0.4815565 | 0.5982281 | -0.6404892 | -0.5077719 | 0.7860942 | 0.3524537 |
| 46 | 400 | C | 9.6392 | 7.1499 | -6.3248 | 0.8470264 | -0.4856701 | 0.2160343 | 0.5152812 | 0.6504438 | -0.5580395 | 0.1305049 | 0.5839926 | 0.8011998 |
| 47 | 412 | C | 11.0167 | 9.5393 | -2.4358 | 0.4843211 | -0.6995943 | -0.5253579 | 0.4863111 | 0.7144422 | -0.5030645 | 0.7272789 | -0.01184264 | 0.6862398 |
| 48 | 424 | C | 4.1256 | 7.1458 | -10.2108 | 0.8660254 | -0.5 | 0.0 | 0.3832907 | 0.663879 | -0.6421471 | 0.3210736 | 0.5561157 | 0.7665814 |
| 49 | 430 | C | -6.8875 | 2.3882 | -6.318 | 0.7440667 | -0.257933 | 0.6163078 | 0.219338 | 0.9656489 | 0.1393308 | -0.631075 | 0.03150831 | 0.7750817 |
| 50 | 442 | C | 2.7662 | 4.7912 | -2.4305 | 0.8660254 | -0.5 | -4.341588e-13 | 0.4641426 | 0.8039185 | -0.3718693 | 0.1859346 | 0.3220482 | 0.9282851 |
| 51 | 448 | C | 0.0 | 0.0 | -21.8897 | 1.0 | 0.0 | 0.0 | 0.0 | 1.0 | 0.0 | 0.0 | 0.0 | 1.0 |
| 52 | 450 | C | 1.3736 | 2.3792 | -17.9928 | 0.8660254 | -0.5 | 0.0 | 0.4097874 | 0.7097726 | -0.5729722 | 0.2864861 | 0.4962084 | 0.8195748 |
| 53 | 456 | C | 5.5058 | 9.5363 | -6.3245 | 0.8660254 | -0.5 | 0.0 | 0.4115927 | 0.7128994 | -0.5677727 | 0.2838864 | 0.4917056 | 0.8231854 |
| 54 | 462 | C | 6.8855 | 11.926 | -2.4371 | 0.8660254 | -0.5 | 0.0 | 0.4256214 | 0.7371979 | -0.524772 | 0.262386 | 0.4544659 | 0.8512428 |
| 55 | 468 | C | -1.3743 | -2.3804 | -14.0938 | 0.8660254 | -0.5 | 0.0 | 0.4858817 | 0.8415718 | -0.2359572 | 0.1179786 | 0.2043449 | 0.9717634 |
| 56 | 474 | C | 6.8981 | 7.1653 | -2.4327 | 0.4747332 | -0.6435709 | -0.6003706 | 0.5845668 | 0.7405083 | -0.3315558 | 0.657959 | -0.1935562 | 0.727754 |
| 57 | 486 | C | 8.27 | 9.5493 | 1.4579 | 0.6931769 | -0.5788765 | -0.4294272 | 0.6532306 | 0.7563564 | 0.0348544 | 0.3046236 | -0.3046753 | 0.9024286 |
| 58 | 498 | C | 4.1497 | 7.1876 | 1.4593 | 0.8660254 | -0.5 | 0.0 | 0.4982796 | 0.8630456 | 0.08288315 | -0.04144157 | -0.07177891 | 0.9965593 |
| 59 | 504 | C | 0.0 | 0.0 | -10.1852 | 1.0 | 0.0 | 0.0 | 0.0 | 1.0 | 0.0 | 0.0 | 0.0 | 1.0 |
| 60 | 506 | C | 5.5116 | 9.5464 | 5.3515 | 0.8660254 | -0.5 | 0.0 | 0.4529617 | 0.7845526 | 0.4234417 | -0.2117209 | -0.3667113 | 0.9059233 |

TABLE S12. Elements of rotation matrix from Cartesian to principal axes of hyperfine tensor with each lattice site for $^{13}$C for the SnV$^{-}$ defect in diamond.
